# Supplementary material for: Causal health impacts of power plant emission controls under modeled and uncertain physical process interference
Source: arXiv:2306.05665 ancillary file (2024-05-14)
Supplement: Supplementary file 1 [file Wikle_Zigler-CausalHealthImpactsOfPowerPlantEmissionControls-SUPPLEMENT.pdf]

Supplementary Material for
"Causal health impacts of power plant emission controls under modeled and uncertain physical process interference."

Nathan B. Wikle[1] and Corwin M. Zigler[2]

[1]Department of Statistics and Actuarial Science, University of Iowa
[2]Department of Statistics and Data Sciences, University of Texas at Austin

January 19, 2024

## Contents

**1 Approximating the Sulfate Model in Discrete Space** **3**

**2 Sulfate Model Diagnostics and Comparisons** **4**

2.1 Model Comparisons and Predictive Diagnostics . . . 4
2.2 Comparing the Sulfate Model to HyADS . . . 7

**3 Assessing Covariate Balance and Overlap** **8**

**4 Stratified Causal Effect Estimates** **14**

4.1 Stratified Estimates for All-Cause Mortality . . . 15
4.2 Stratified Estimates for Asthma ED Visits . . . 16

**5 Inference via Bayesian Modularization** **17**

5.1 Overview . . . 17
5.2 Including Uncertainty in $G$: A Simulation Study . . . 18
5.3 Simulation Study Results . . . 22
5.3.1 Estimating Bias, Coverage, and Proportion of Variance . . . 22
5.3.2 Major Findings . . . 23
5.3.3 Results: CM1 . . . 27
5.3.4 Results: CM2 . . . 30
5.3.5 Results: CM3 . . . 33
5.3.6 Results: PM1 . . . 36
5.3.7 Results: PM2 . . . 39
5.3.8 Results: PM3 . . . 42

**6 Log-linear BART Tuning Parameters** **45**
6.1 Number of Trees . . . . . 45
6.2 The Tree Prior: Splitting Rules . . . . . 48
6.3 Leaf Prior Tuning Parameter . . . . . 52

**7 Estimated Upwind Effects Without Key-Associated Treatment** **53**

**8 Testing for Spatial Autocorrelation** **56**

# 1 Approximating the Sulfate Model in Discrete Space

Section 4 of the primary text describes the mechanistic model of annual sulfate concentrations in the US. We briefly describe the discretization of the continuous-space SPDE,

$$\mathrm{d}\nu(\boldsymbol{s},t) = \big( - \mathcal{L}_{\boldsymbol{\theta}}(\boldsymbol{s},t)\, \nu(\boldsymbol{s},t) + R_{\boldsymbol{\theta}}(\boldsymbol{s},t)\big)\mathrm{d}t \tag{SM.1}$$

$$\mathrm{d}\eta(\boldsymbol{s},t) = \big( - \mathcal{A}_{\boldsymbol{\theta}}(\boldsymbol{s},t)\, \eta(\boldsymbol{s},t) + \theta_3\, \nu(\boldsymbol{s},t)\big)\mathrm{d}t + \xi(\boldsymbol{s},t), \tag{SM.2}$$

into a discrete-space stochastic differential equation (SDE). A more comprehensive overview can be found in [26].

The SPDE in (SM.1) and (SM.2) is challenging to solve. A solution to this problem, as outlined by [26], is to approximate (SM.1) and (SM.2) in discrete space. Instead of solving the SPDE on a continuous spatial region $\mathcal{D}$, we instead restrict our focus to a grid of spatial locations, $D = \{\boldsymbol{s}_1, \dots, \boldsymbol{s}_n\}$. In our analysis, the locations in $D$ correspond to the raster elements of the sulfate data. Then, if $\boldsymbol{\nu}_t = (\nu(\boldsymbol{s}_1,t), \dots, \nu(\boldsymbol{s}_n,t))'$ and $\boldsymbol{\eta}_t = (\eta(\boldsymbol{s}_1,t), \dots, \eta(\boldsymbol{s}_n,t))'$ denote the vectorized versions of $SO_2$ and ${SO_4}^{2-}$ at time $t$, we can represent (SM.1) and (SM.2) in discrete space as

$$\mathrm{d}\boldsymbol{\nu}_t = \big( - \boldsymbol{L}_{\boldsymbol{\theta}}\, \boldsymbol{\nu}_t + \boldsymbol{R}_{\boldsymbol{\theta},t}\big)\mathrm{d}t, \tag{SM.3}$$

$$\mathrm{d}\boldsymbol{\eta}_t = \big( - \boldsymbol{A}_{\boldsymbol{\theta}}\, \boldsymbol{\eta}_t + \theta_3\, \boldsymbol{\nu}_t\big)\mathrm{d}t + \mathrm{d}\boldsymbol{W}_t. \tag{SM.4}$$

In addition to the vectorization of $\boldsymbol{\nu}_t$ and $\boldsymbol{\eta}_t$, the advection-diffusion operators $\mathcal{L}_{\boldsymbol{\theta}}$ and $\mathcal{A}_{\boldsymbol{\theta}}$ have been replaced with their finite volume method (FVM) (matrix) approximations, $\boldsymbol{L}_{\boldsymbol{\theta}}$ and $\boldsymbol{A}_{\boldsymbol{\theta}}$; the $SO_2$ source term $R_{\boldsymbol{\theta}}(\boldsymbol{s},t)$ has been exchanged for its vectorized version, $\boldsymbol{R}_{\boldsymbol{\theta},t}$; and the space-time noise process, $\xi(\boldsymbol{s},t)$, has been replaced with $\mathrm{d}\boldsymbol{W}_t$, the distributional derivative of an $n$-dimensional Brownian motion, $\boldsymbol{W}_t = (W(\boldsymbol{s}_1,t), \dots, W(\boldsymbol{s}_n,t))'$.

The motivation behind this numerical discretization is the convenient representation of the SPDE in (SM.2) as an SDE in (SM.4) — in particular, a multivariate Ornstein-Uhlenbeck (OU) process [24]. [26] show that, under certain stationarity assumptions, (SM.4) defines three useful probabilistic models for spatial data observed from linear dynamical systems. When the data are time-averaged realizations of the process, as is the case with the observed annual average ${SO_4}^{2-}$ concentrations, the appropriate likelihood model is a Gaussian distribution where the mean, $\boldsymbol{\mu}_{\boldsymbol{\theta}}(\boldsymbol{R})$, is the time-limiting deterministic solution to (SM.3, SM.4) under emissions scenario $\boldsymbol{R}$, and the precision matrix, $\boldsymbol{\Sigma}_{\boldsymbol{\theta}}^{-1}$, is proportional to the crossproduct of the linear operator $\boldsymbol{A}_{\boldsymbol{\theta}}$. Thus, the model for annual average ${SO_4}^{2-}$, which we denote with $\bar{\boldsymbol{\eta}}$, is

$$\bar{\boldsymbol{\eta}} \sim N\bigg(\beta_0 + \boldsymbol{\mu}_{\boldsymbol{\theta}}(\boldsymbol{R}),\, \boldsymbol{\Sigma}_{\boldsymbol{\theta}}\bigg), \tag{SM.5}$$

where

$$\boldsymbol{\mu}_{\boldsymbol{\theta}}(\boldsymbol{R}) = \theta_3 \boldsymbol{A}_{\boldsymbol{\theta}}^{-1} \boldsymbol{L}_{\boldsymbol{\theta}}^{-1} \boldsymbol{R}, \quad \boldsymbol{\Sigma}_{\boldsymbol{\theta}} = \frac{\sigma^2}{T} (\boldsymbol{A}_{\boldsymbol{\theta}}' \boldsymbol{A}_{\boldsymbol{\theta}})^{-1}, \tag{SM.6}$$

and $\beta_0$ represents a constant source of "background" ${SO_4}^{2-}$, which accounts for emissions sources outside the study area. We set $T = 1$ to denote the average of $\boldsymbol{\eta}_t$ over one year. Note that (SM.5) is a simultaneous autoregressive (SAR) model for discrete spatial data [25], where the (sparse) precision matrix $\boldsymbol{\Sigma}_{\boldsymbol{\theta}}^{-1}$ is determined by the advection-diffusion process $\boldsymbol{A}_{\boldsymbol{\theta}}$. Table SM.1 contains a description

of the components of $\boldsymbol{\theta}$, their prior distributions, and summaries of the inferred marginal posterior distributions.

**Table SM.1:** Parameter estimates and priors for $\boldsymbol{\theta}$ and $\beta_0$. Unit of time $T = 1$ year.

| Parameter | Interpretation | $\hat{\boldsymbol{\theta}} \approx \mathrm{E}(\boldsymbol{\theta}\|\boldsymbol{Y})$ | 95% Credible Interval | Prior |
|---|---|---|---|---|
| $\theta_1$ | rate of sub-annual wind transport | 2647 | (1515, 3890) | Half-Normal($\sigma = 1 \times 10^4$) |
| $\theta_2$ | rate of annual wind transport | 15.2 | (0.34, 60.48) | Half-Normal($\sigma = 1 \times 10^3$) |
| $\theta_3$ | $SO_2 \rightarrow {SO_4}^{2-}$ | 169.1 | (1.3, 1045.4) | Exponential($\lambda = 0.01$) |
| $\theta_4$ | proportional rate of $SO_2$ emission | 2.60 | (0.30, 7.70) | Half-Normal($\sigma = \sqrt{10}$) |
| $\sigma^2$ | B.M. process variance | 49600 | (15800, 99600) | Exponential($\lambda = 0.001$) |
| $\beta_0$ | constant source of "background" ${SO_4}^{2-}$ | 0.64 | (0.03, 0.95) | Half-Normal($\sigma = \sqrt{5}$) |
| $\delta$ | deposition of ${SO_4}^{2-}$ | NA | NA | fixed at 50 |

# 2 Sulfate Model Diagnostics and Comparisons

## 2.1 Model Comparisons and Predictive Diagnostics

Given the fundamental role of the sulfate model's (mechanistic) mean structure in defining $T$ and $G_i$, we focus on evidence of its potential misspecification. To do so, we first performed a model comparison between the fitted sulfate model and three alternatives. Each model is of the form,

$$\boldsymbol{y} \sim N\big(\boldsymbol{\mu}_i, \boldsymbol{\Sigma}_{\boldsymbol{\theta}}\big), \tag{SM.7}$$

where $\boldsymbol{y}$ denotes the annual average sulfate concentrations and $\boldsymbol{\Sigma}_{\boldsymbol{\theta}}$ is the simulataneous autoregressive (SAR) covariance matrix described in [26] for advection-diffusion processes. However, the specification of the mean, $\boldsymbol{\mu}_i$, varies between the four models:

- The original model: $\boldsymbol{\mu}^* = \beta_0 + \mu_{\boldsymbol{\theta}}(\boldsymbol{R}_{full})$,
- Alternative 1: $\boldsymbol{\mu}_1 = \beta_0 + \mu_{\boldsymbol{\theta}}(\boldsymbol{R}_{USA})$,
- Alternative 2: $\boldsymbol{\mu}_2 = \mu_{\boldsymbol{\theta}}(\boldsymbol{R}_{full})$,
- Alternative 3: $\boldsymbol{\mu}_3 = \mu_{\boldsymbol{\theta}}(\boldsymbol{R}_{USA})$.

In all cases, $\mu_{\boldsymbol{\theta}}$ denotes the deterministic solution to the specified advection-diffusion process (i.e., Equation SM.6 in the Supplement); the key differences are (i) the inclusion (or exclusion) of $\beta_0$, an intercept term meant to account for unspecified "background" sources of sulfate, particularly those coming from sources located outside the study region, and (ii) the use of coal power plant emissions from only the United States ($\boldsymbol{R}_{USA}$), or emissions sources from both the USA and Mexico ($\boldsymbol{R}_{full}$). A visual comparison of the estimated posterior mean $SO_4$ surfaces across the four models shows that the inclusion of $\beta_0$ in $\boldsymbol{\mu}_i$ results in sulfate concentrations that are more concentrated around power plant facilities, which is inline with estimates of power plant-attributed sulfate from deterministic models. Similarly, the use of Mexican emissions data — originally motivated by the large amount of sulfate observed near the Mexico-Texas border — results in higher estimated sulfate concentrations in both Mexico and Texas. Table SM.2 shows a comparison of the deviance information criterion (DIC) [22], posterior predictive loss (PPL) [11], and multivariate energy score [12] of the four fitted models. The model used in the paper, which includes both $\beta_0$ and $\boldsymbol{R}_{full}$, outperforms the alternatives across the three metrics.

**Table SM.2:** A comparison between the original model and three alternatives using (a) deviance information criterion (DIC), (b) posterior predictive loss (PPL), and (c) the multivariate energy score.

| Model | DIC | PPL | Energy Score |
|---|---|---|---|
| Original | **-82272.99** | **2270.85** | **30.45** |
| Alternative 1 | -82115.31 | 3024.09 | 35.97 |
| Alternative 2 | -82143.40 | 2815.28 | 34.48 |
| Alternative 3 | -82078.73 | 2880.87 | 38.17 |

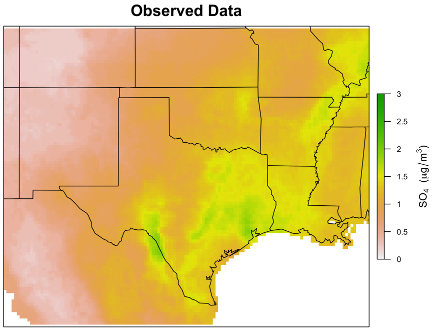


**(a)** The observed sulfate data, $\boldsymbol{y}$

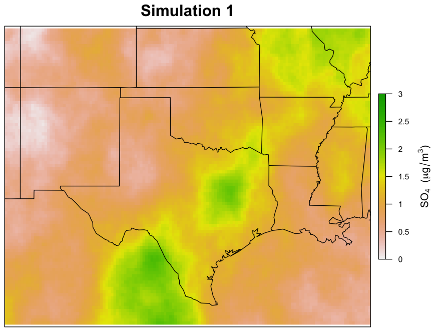


**(b)** Predictive simulation, $\boldsymbol{y}_1^{rep}$.

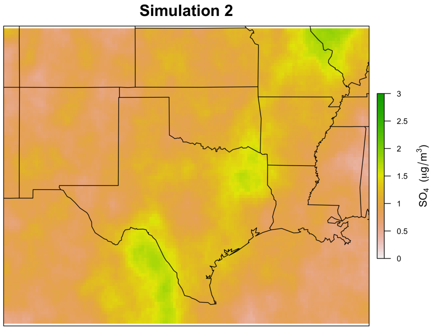


**(c)** Predictive simulation, $\boldsymbol{y}_2^{rep}$.

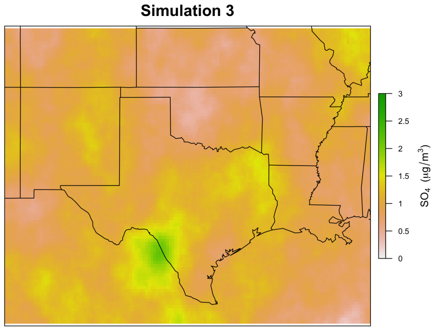


**(d)** Predictive simulation, $\boldsymbol{y}_3^{rep}$.

**Figure 1:** A comparison of the observed sulfate data with three simulations from the posterior predictive distribution.

In addition to model comparisons, we performed a series of posterior predictive checks to investigate how well our sulfate model represents the real-world process of interest. Figure 1 shows the observed sulfate data, $\boldsymbol{y}$, along with three simulations from the posterior predictive distribution,

$$\boldsymbol{y}^{rep} \sim p(\boldsymbol{y}^{rep}|\boldsymbol{y}) \equiv \int p(\boldsymbol{y}^{rep}|\boldsymbol{\theta})p(\boldsymbol{\theta}|\boldsymbol{y})d\boldsymbol{\theta}. \tag{SM.8}$$

We used three discrepancy measures to assess model fit: (i) sample mean, $T_1(\boldsymbol{y}) = \bar{\boldsymbol{y}}$, (ii) sample variance, $T_2(\boldsymbol{y}) = s_y^2$, and (iii) marginal sulfate concentration, $T_3(y_i) = y_i$. Figure 1 shows a comparison of the posterior predictive distributions of $T_1(\boldsymbol{y})$ and $T_2(\boldsymbol{y})$ (using 1000 posterior predictive simulations) against the observed data (represented by a red vertical line). Notice that the predictive distributions overlap with observed data for both $T_1$ and $T_2$, with predictive $p$-values of 0.308 and 0.884 for the mean and variance discrepancies, respectively. In other words, there is not evidence of a significant difference between the observed and predictive distributions when considering discrepancies which ignore spatial dependence.

However, the predictive $p$-values for $T_3(\boldsymbol{y}) = y_i$, the marginal values of $\boldsymbol{y}$, indicate regions in

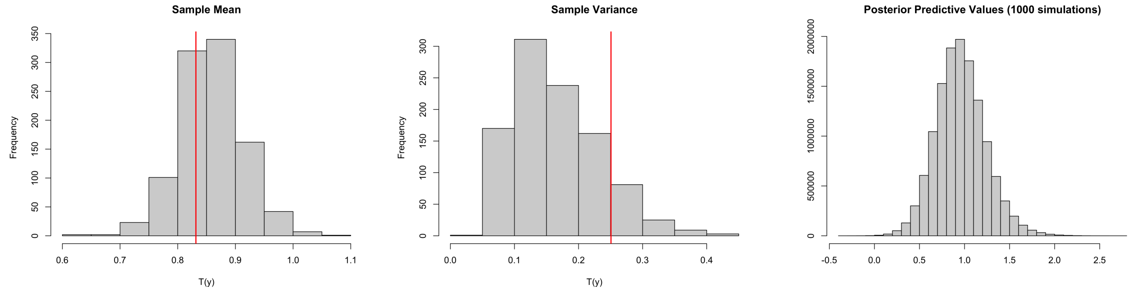


**(a)** $T(\boldsymbol{y}) = \bar{\boldsymbol{y}}$ **(b)** $T(\boldsymbol{y}) = s_y^2$. **(c)** Values of $y_i^{rep}$ (1000 sims).

**Figure 2:** A comparison of summary statistics calculated with from the posterior predictive distribution with that of the observed data, including (a) sample mean, (b) sample variance, and (c) the distribution of marginal values of $y_i$.

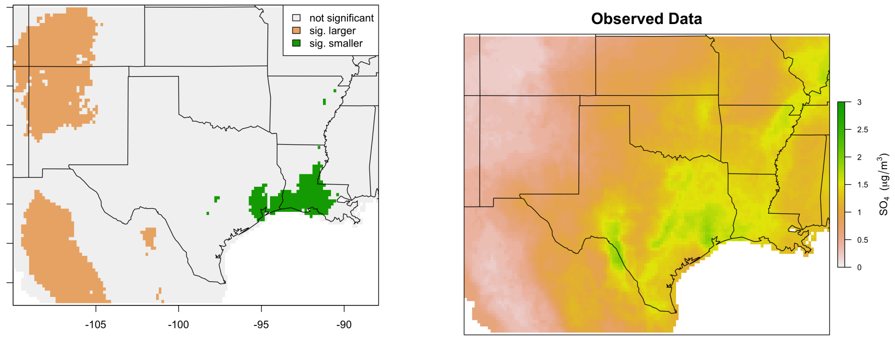


**(a)** Significant differences in the marginal discrepancy, $T_3(y_i)$. **(b)** Observed sulfate.

**Figure 3:** A figure showing (a) regions in which the marginal posterior predictive distribution is either significantly ($\alpha = 0.05$) larger or greater than the observed data, and (b) the observed sulfate surface.

which the modeled and observed process are significantly different. Figure 3 shows regions in which the predictive distribution is significantly higher (shown in orange, $\alpha = 0.05$) and significantly lower (shown in green) than the observed data. These departures are likely due to the omission of non-power plant sources of sulfate in our model (e.g., from industrial sources and shipping traffic along the Gulf Coast); they may also indicate that the model's advection-diffusion process is unable to accommodate certain complexities in the pollution transport process, such as potential process heterogeneity seen at higher elevations in the western region of our study.

To further assess the consequences of the potential misspecification of the transport process, we compared the estimated sulfate emissions due to power plants with those from HyADS (the HYSPLIT average dispersion model) — a deterministic, reduced complexity model of pollution transport [13]. This comparison (see Section 2 of the Supplement) finds that the two models identify similar regions with high pollution concentration attributable to power plant emissions. In general, the statistical model's estimates are both larger in magnitude and more spatially smooth than the HyADS output. However, the *relative* contribution of a given power plant to the overall pollution concentration is similar across models. Thus, the normalized exposure levels, $G_i$, are similar when using either the statistical or deterministic model; this gives us some confidence that our chosen exposure model is not unreasonable.

Finally, note that the normality assumption for our model is a consequence of the specification of the noise process in the SPDE (i.e., Equations (4) and (5)). Although this assumption could

be problematic in areas with small amounts of pollution concentration (e.g., the western region of our study, as shown in Figure 3a), we believe it is a reasonable assumption given the magnitude of the concentrations considered in this study. For example, Figure 2c shows a histogram of the simulated marginal sulfate concentrations from 1000 draws of the posterior predictive distribution. Of the almost 13 million simulated values, only 0.02% of them are negative. Similarly, the only regions in which the estimate mean surface of $SO_4$ attributed to power plant emissions is larger than the observed sulfate concentrations are in regions outside of Texas. Thus, we do not believe this to be a major concern for the specification of the exposure model in Texas, although relaxing this assumption for the advection-diffusion processes considered here and in [26] could be an interesting area of future work.

## 2.2 Comparing the Sulfate Model to HyADS

As described in the primary text, the fitted sulfate model (SM.5) (which we will hereafter refer to as the OU model) is used to generate upwind treatment exposure levels, $G_i$; the utility of the exposure level is dependent on the model's ability to predict the proportion of sulfate concentration attributable to an emissions source. Consequently, we compared the model's predicted sulfate concentrations attributable to the observed coal-fired power plant $SO_2$ emissions in 2016 with output from HyADS (the HYSPLIT average dispersion model), a deterministic, reduced-complexity model linking pollution exposure to power plant emissions [13].

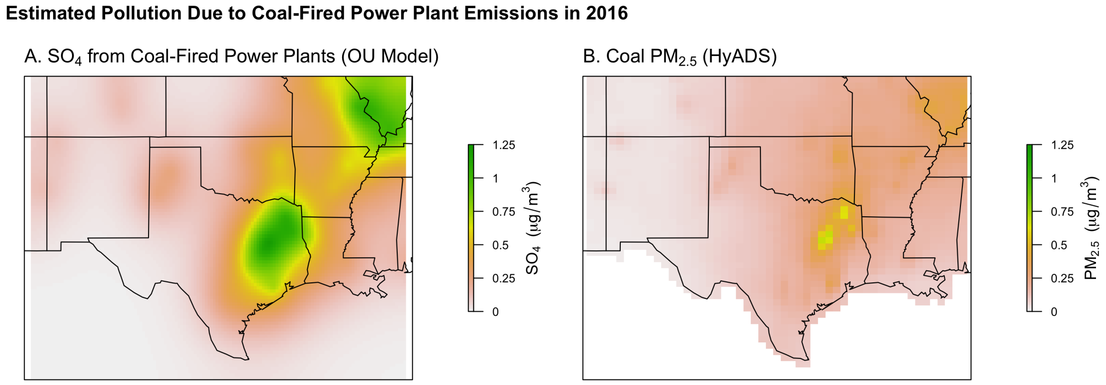


**Figure 4:** A comparison of the estimated pollution concentrations attributable to coal-fired power plant emissions in 2016, using (A) the (statistical) OU model, and (B) the (deterministic) HyADS model.

Figure 4 shows (A) the OU model's estimated posterior mean sulfate surface attributable to the reported coal-fired power plant $SO_2$ emissions in 2016, compared with (B) the HyADS model's predicted coal $PM_{2.5}$ concentrations, the concentration of $PM_{2.5}$ attributable to coal-fired power plant emissions (note that the majority of coal $PM_{2.5}$ is sulfate). In general, the models identify similar regions with high pollution concentrations due to power plant emissions (see, for example, eastern Texas, or the confluence of the Ohio and Mississippi River in the northeast corner of the study region). However, in general, the OU model's estimates are both larger in magnitude and more spatially smooth than the HyADS output.

Recall that the analysis of causal effects does not rely on accurate prediction of the *level* of $SO_4$, but rather the characterization of the relative influences encoded in the weighted bipartite

adjacency matrix $T$. Essentially, the quantity $G_i$ is defined as the *weighted* proportion of scrubbed upwind facilities, where the weight, $T_{ij}/T^*_{i\cdot}$ is defined as the proportion of $SO_4{}^{2-}$ in ZCTA $i$ that is attributable to 1000 tons $SO_2$ emitted from facility $j$ (see Section 4.2). Thus, a more pertinent comparison is that of the *relative* contribution of power plant $j$ to the expected pollution concentration. Figure 5 shows the estimated proportion of 2016 coal pollution concentrations attributable to emissions from the Big Brown Power Plant, Fairfield, TX. Once again, the OU-derived surface is more spatially smooth than the HyADS surface. However, the *magnitude* of the relative proportion of coal-derived pollutants is very similar across models (OU maximum proportion = 0.40 , HyADS maximum proportion = 0.43). In other words, the exposure levels, $G_i$, generated with HyADS would be very similar to the exposure levels generated with the OU model (albeit without the uncertainty quantification provided by the OU model). Note that the HyADS model is itself a reduced complexity air quality model relying primarily on $SO_2$ emissions and historical wind fields, with limited use of observed sulfate data. Thus, HyADS should not be regarded as a form of "ground truth," just as a comparator with the statistical OU model.

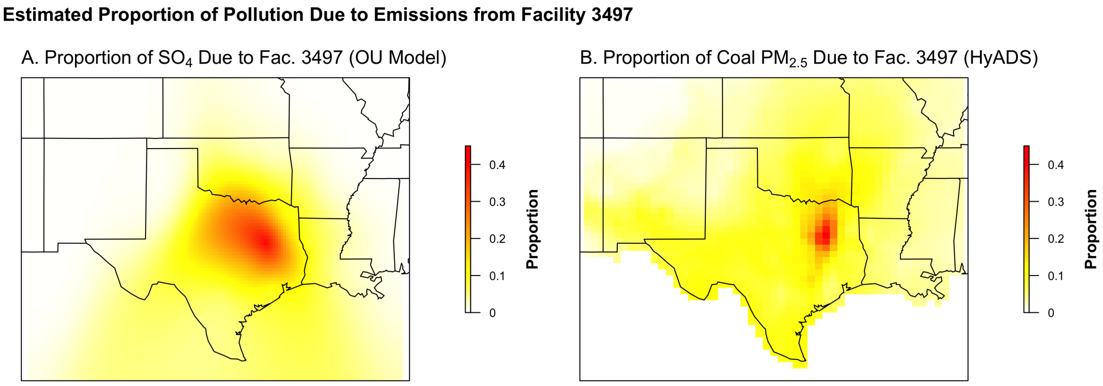


**Figure 5:** A comparison of the estimated proportion of pollution attributable to coal-fired power plant emissions from Facility 3497 (Big Brown Power Plant, Fairfield, TX), using (A) the (statistical) OU model, and (B) the (deterministic) HyADS model.

# 3 Assessing Covariate Balance and Overlap

One drawback to causal effect estimation with BART is its inability to easily quantify covariate balance and overlap. To better understand the distribution of covariates across treatment levels, we compared covariate balance when using propensity score weighting. Balance assessment was performed marginally — once using propensity scores fitted to the key-associated treatment, $Z_i$, and once using generalized propensity scores fitted to the (mean) upwind treatment level, $G_i = \bar{g}_i$. For binary treatment $Z_i$, balance was assessed using the absolute standardized mean difference [2] between treated ($Z = 1$) and untreated ($Z = 0$) units; propensity scores were estimated using (i) BART and (ii) covariate balancing propensity scores (CBPS) [14]. For continuous treatment $G_i$, balance was assessed with the (weighted) Pearson correlation between covariate and treatment [3]; generalized propensity scores were estimated using (i) BART and (ii) CBPS [9].

The balance assessment results are shown in Figures 6 and 8. For $Z_i$, the weighted standardized mean differences using the CBPS are often substantially lower than the unweighted or BART-based mean differences. Moreover, 23 of the 26 covariates have CBPS-weighted differences that are below 0.1. Similarly, when comparing balance for $G_i$, the CBPS-weighted correlations are very low (25/26 below 0.1), often improving on the BART and unweighted correlations. Based on these assessments, we conclude that covariate balance can be achieved, conditional on adjustment with an appropriate choice of propensity score. Furthermore, Figures 7 and 9 show a considerable amount of propensity score overlap across treatment groups. These results give us greater confidence that causal effects estimated with a log-linear BART outcome model may be less susceptible to extrapolation due to lack of overlap in the covariate space. In sparse regions of the covariate space, the estimated log-linear BART dose-response function will be influenced by the prior, with correspondingly large uncertainty bounds.

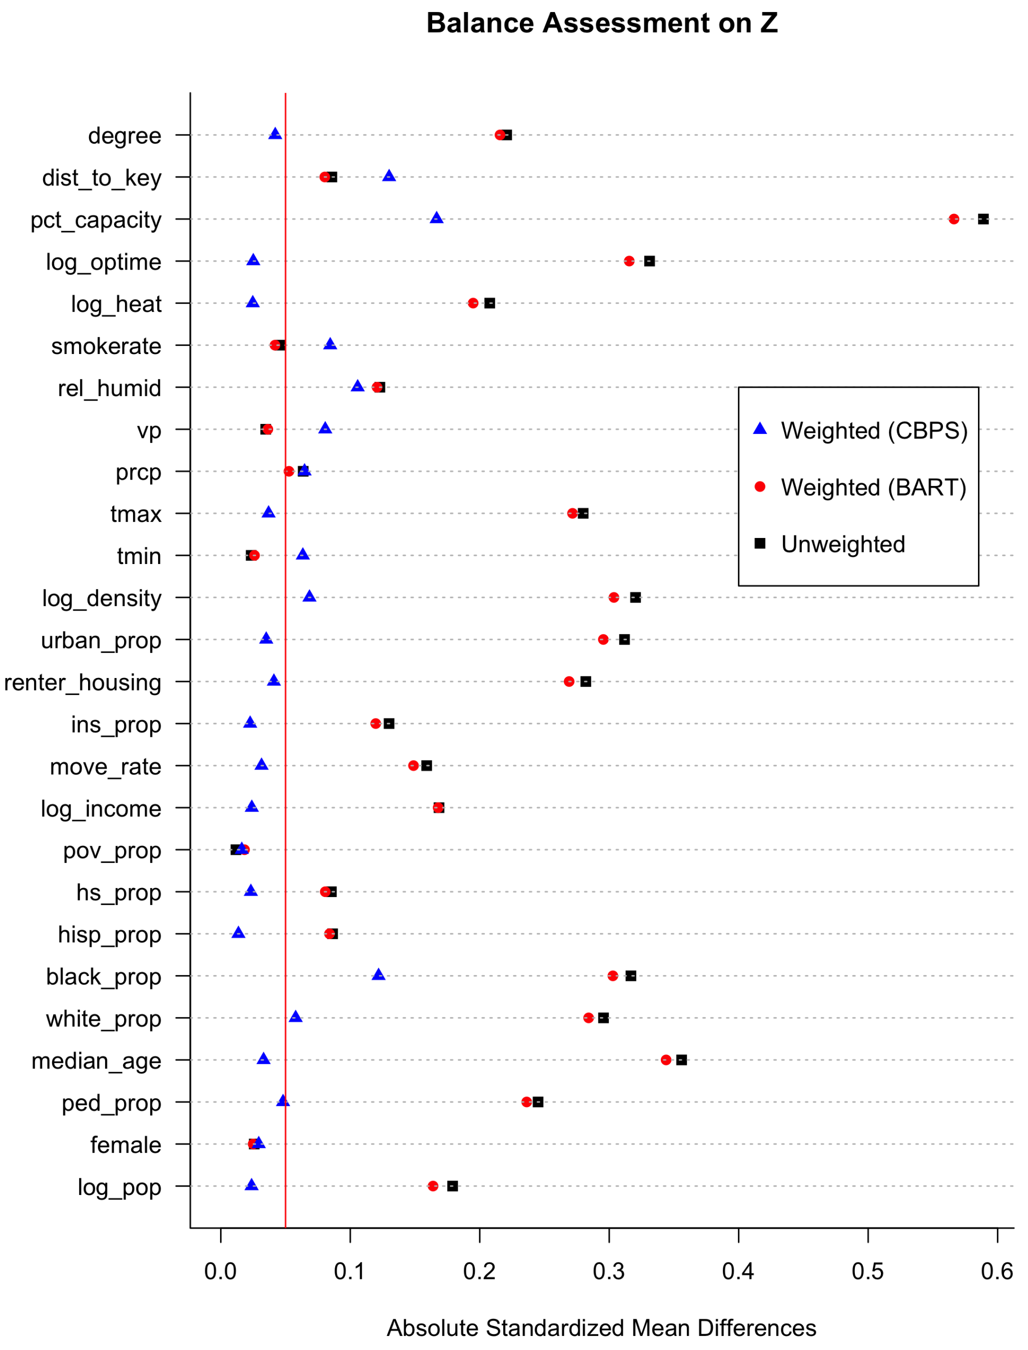


**Figure 6:** A comparison of the absolute standardized mean difference between treated ($Z = 1$) and untreated ($Z = 0$) units, including the weighted difference when using propensity scores estimated with BART and CBPS.

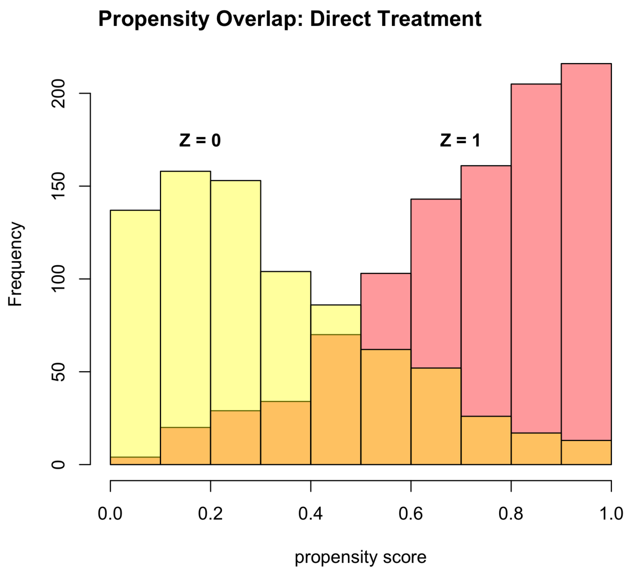


**Figure 7:** A comparison of propensity score overlap (using CBPS) between treated $(z = 1)$ and untreated $(z = 0)$ units.

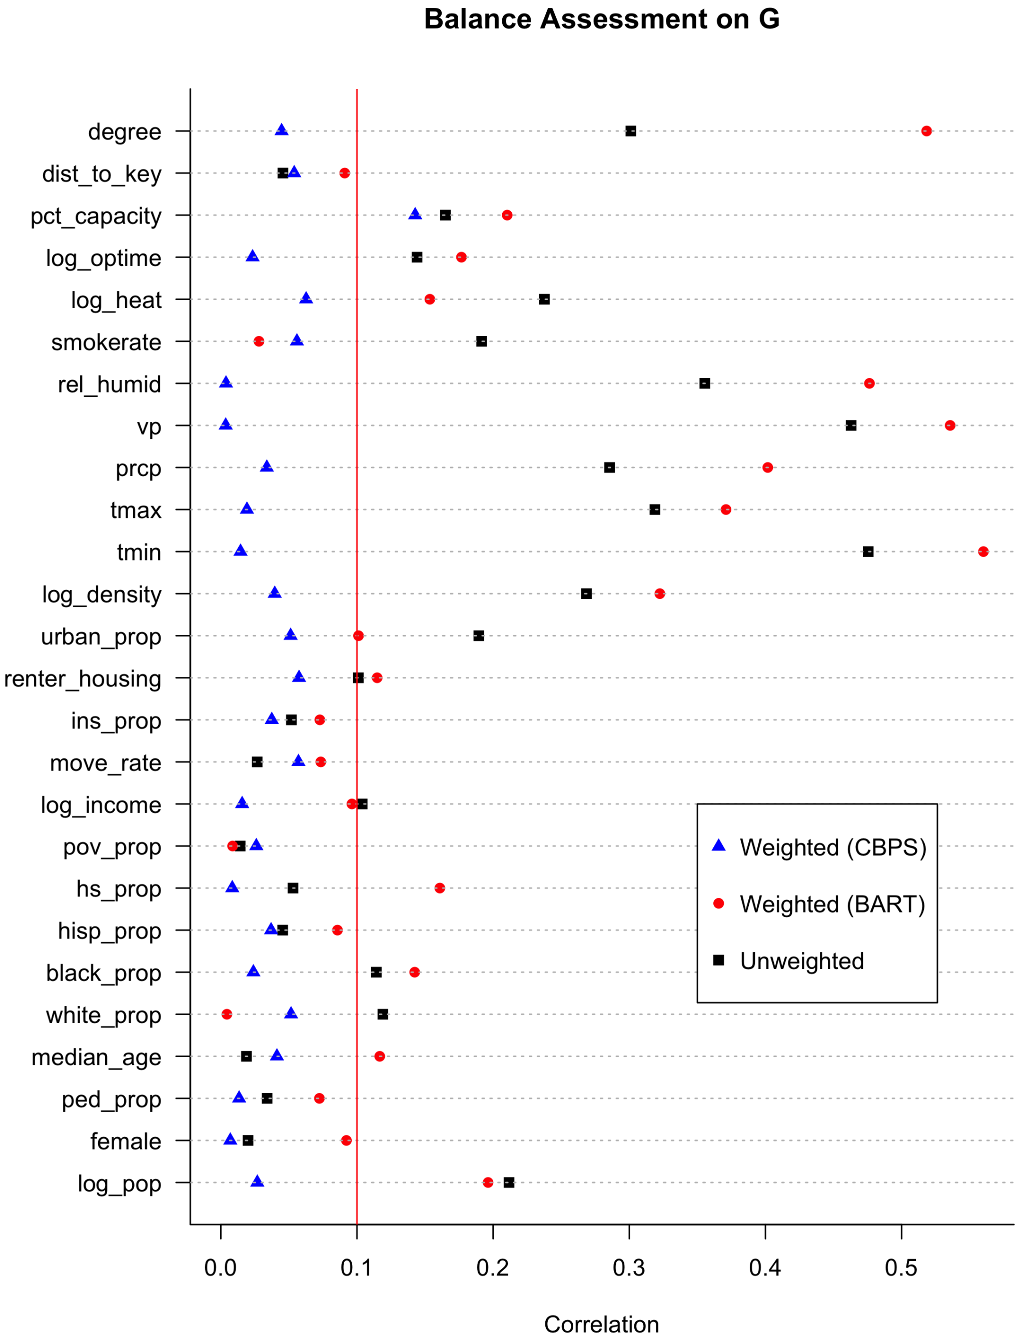


**Figure 8:** A comparison of the Pearson correlation between covariate and treatment ($G = g$), with generalized propensity scores estimated with BART and CBPS.

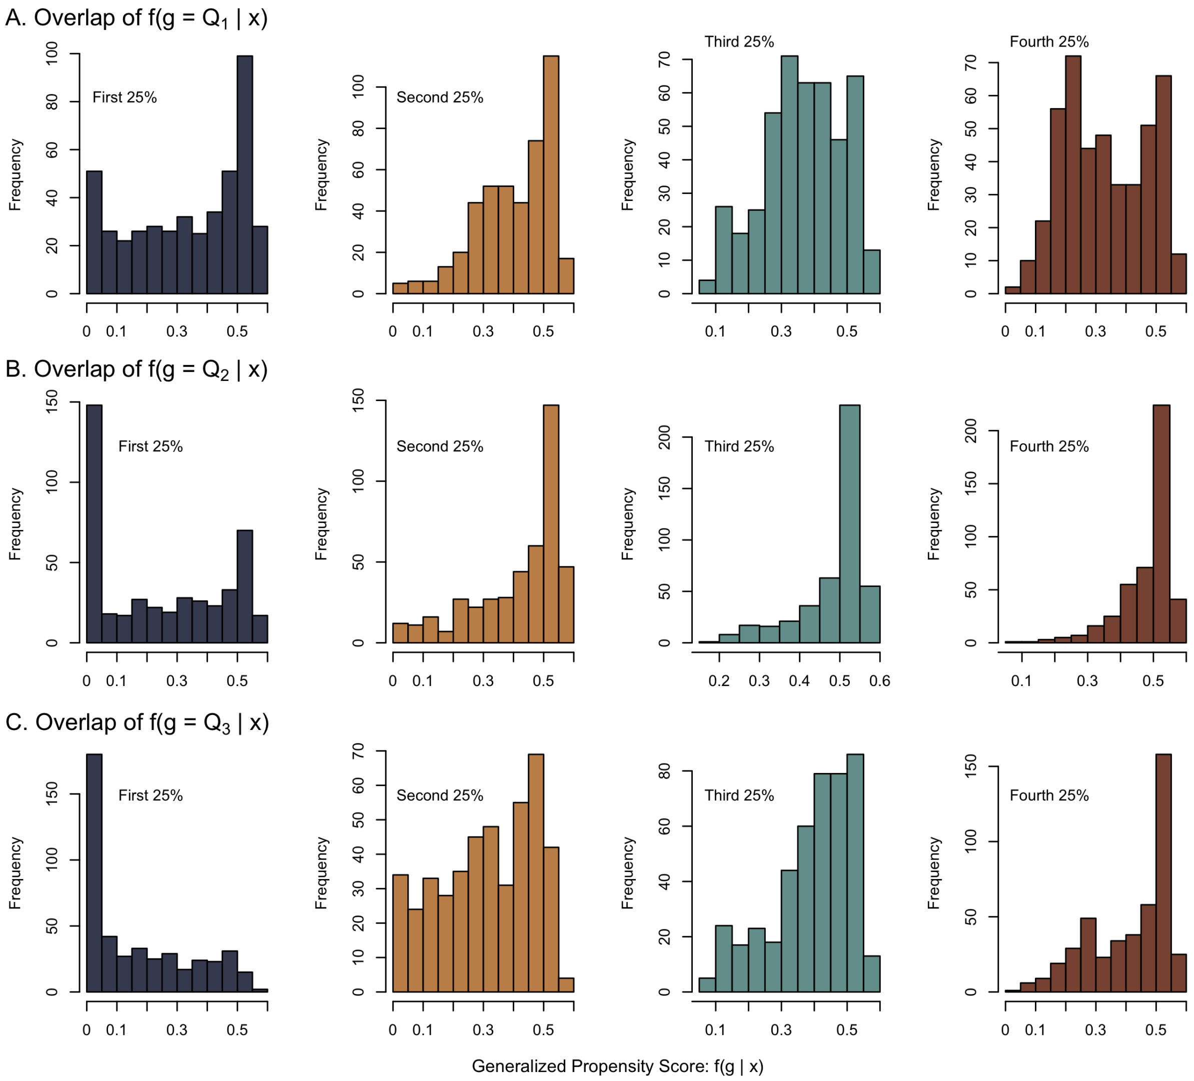


**Figure 9:** A comparison of generalized propensity score overlap (using CBPS), for three different evaluations of $f(g|x)$ (at the 1st, 2nd, and 3rd quantiles of $g$) compared across four blocks of $g$ (1st 25%, 2nd 25%, 3rd 25%, and 4th 25% of the data).

# 4 Stratified Causal Effect Estimates

In addition to the causal effect estimates described in Section 7 of the primary text, which compared the estimated direct and indirect effects estimated from all Texas ZCTAs, we considered effect estimates across different ZCTA strata. These include comparisons based on $\bar{T}^*_{i\cdot}$, the (weighted) degree of node $i$, for three strata: low, medium, and high, as well as comparisons based on the distance of the centroid of each $ZCTA$ from its key-associated power plant, stratified into four groups: [0, 50 km), [50, 100 km), [100, 200 km), and 200+ km. The corresponding effect estimates are shown in Figures 10 and 11. The results are largely the same across strata, indicating that the effect of scrubbers is relatively homogeneous across degree (a measure of the total influence of surrounding power plant facilities) and ZCTA distance to key-associated facilities.

## 4.1 Stratified Estimates for All-Cause Mortality

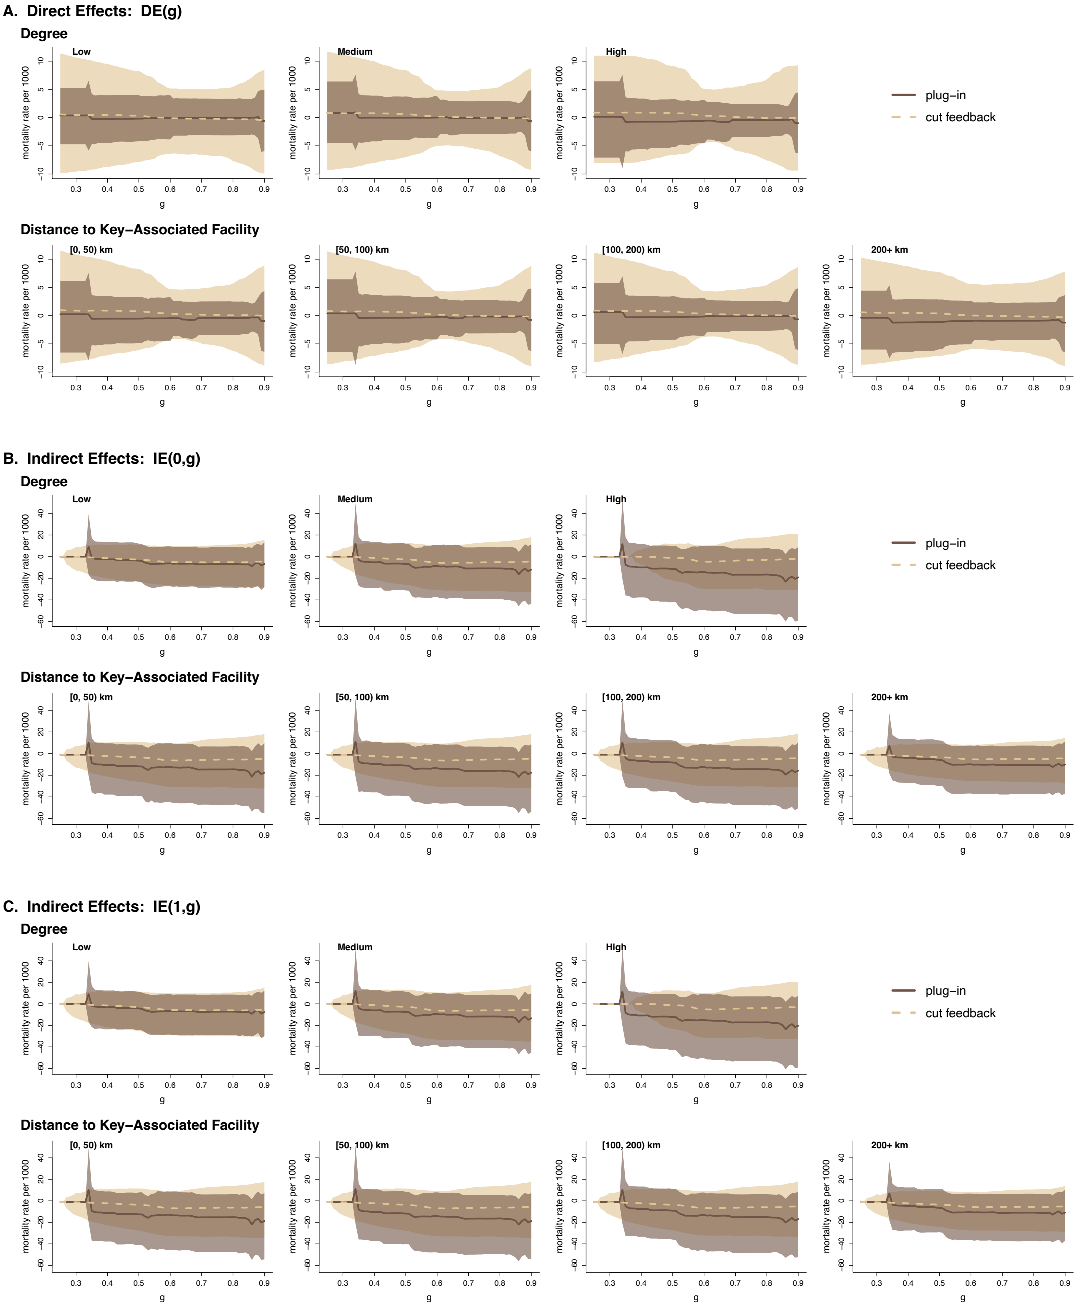


**Figure 10:** Estimated causal effects from the all-cause mortality analysis, stratified by degree and distance to key-associated facility.

## 4.2 Stratified Estimates for Asthma ED Visits

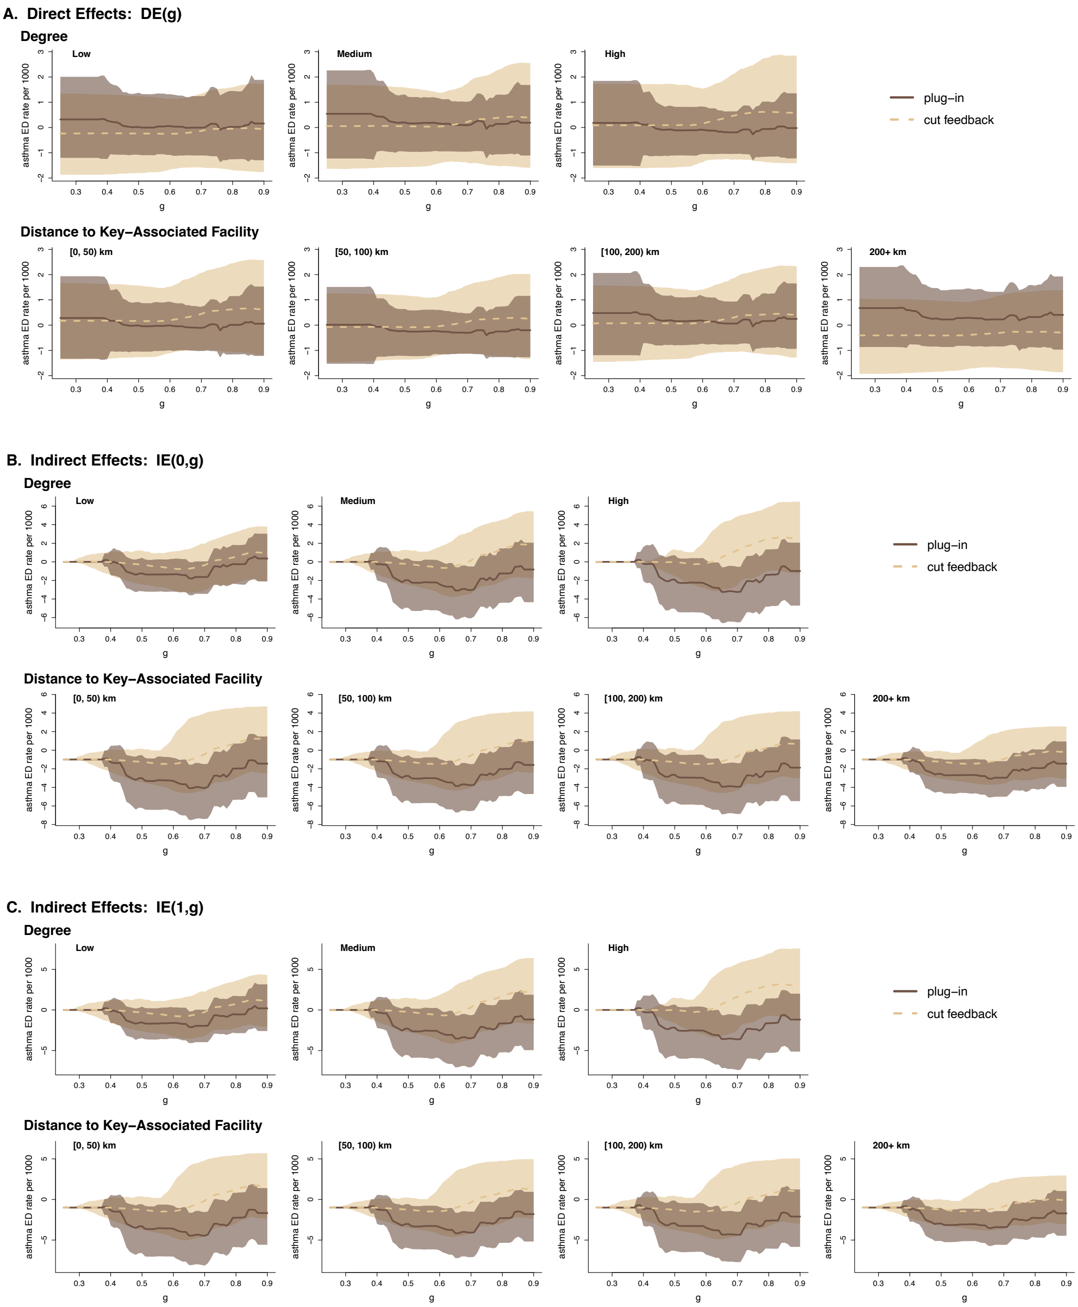


**Figure 11:** Estimated causal effects from the pediatric asthma ED visit analysis, stratified by degree and distance to key-associated facility.

## 5 Inference via Bayesian Modularization

### 5.1 Overview

As discussed in Section 6, some care must be taken when jointly estimating the interference structure and causal effects. Following the notation of the manuscript, let $\boldsymbol{y}$ denote the observed health outcome data, $\boldsymbol{\alpha}$ the health outcome model parameters, $\bar{\boldsymbol{\eta}}$ the sulfate data (used to estimate the interference structure), and $\boldsymbol{\theta}$ the sulfate model parameters (i.e., the parameters which determine the estimated interference structure). Unfortunately, inference from the joint Bayesian hierarchical posterior distribution,

$$\pi(\boldsymbol{\alpha}, \boldsymbol{\theta} \mid \boldsymbol{y}, \bar{\boldsymbol{\eta}}) = \pi(\boldsymbol{\alpha} \mid \boldsymbol{y}, \boldsymbol{\theta})\pi(\boldsymbol{\theta} \mid \boldsymbol{y}, \bar{\boldsymbol{\eta}}), \tag{SM.9}$$

may result in information from $\boldsymbol{y}$ influencing the estimates of $\boldsymbol{\theta}$. In other words, the health outcome data may potentially influence the inferred interference structure, and ultimately the estimated upwind treatment exposure levels, $G$. As discussed in Section 5, the sulfate model — and the corresponding interference structure — was based on our underlying knowledge of the physical sulfate transport process. Consequently, unwanted "feedback" from the health outcome data to the treatment model is conceptually perverse, as the treatment should naturally be assigned independent of the outcome.

To avoid this unwanted model feedback, we consider a *modular* approach to Bayesian inference, in which the interference structure (i.e., the sulfate model) is estimated without inclusion of the health outcomes data. Bayesian modularization schemes can be found in many applied settings. In the context of air pollution, environmental health studies sometimes use air pollution exposure estimates as inputs in a separate model for health outcomes; recent work has focused on how uncertainty in the exposure estimates might be propagated to the outcome model [6, 16, 8]. Similarly, the notion of "cutting feedback" [20] between outcome and treatment assignment has proved central to Bayesian propensity score estimation [28, 29, 23], while early Bayesian modularization efforts can be found in the pharmacokinetic-pharmacodynamic (PKPD) literature [17, 20].

**Algorithm 1** Cutting Feedback

Fit the sulfate model, $\pi(\boldsymbol{\theta}|\bar{\boldsymbol{\eta}})$.
**for** $k = 1, \ldots,$ K **do** ▷ *i.e., a multiple imputation approach.*
  Sample $\boldsymbol{\theta}^{(k)} \sim \pi(\boldsymbol{\theta}|\bar{\boldsymbol{\eta}})$.
  Generate samples, $\boldsymbol{\alpha}^{(ki)} \sim \pi(\boldsymbol{\alpha}|\boldsymbol{y}, \boldsymbol{\theta}^{(k)})$, $i = 1, \ldots, n_k$.
**end for**
Pool the $\boldsymbol{\alpha}^{(ki)}$ MCMC samples. ▷ *Pooled samples are from* $\pi^*(\boldsymbol{\alpha}) = \int \pi(\boldsymbol{\alpha}|\boldsymbol{y}, \boldsymbol{\theta})\pi(\boldsymbol{\theta}|\bar{\boldsymbol{\eta}})d\boldsymbol{\theta}$.

Despite the prevalence of Bayesian modularization, there remains no consensus as to how uncertainty from one module should be propagated to the next [4, 15, 8]. In our analysis, we consider an estimator with inference based on the "cut function,"

$$\pi^*(\boldsymbol{\alpha}, \boldsymbol{\theta} \mid \boldsymbol{y}, \bar{\boldsymbol{\eta}}) = \pi(\boldsymbol{\alpha} \mid \boldsymbol{y}, \boldsymbol{\theta})\pi(\boldsymbol{\theta}|\bar{\boldsymbol{\eta}}), \tag{SM.10}$$

i.e., the dependence of $\boldsymbol{\theta}$ on $\boldsymbol{y}$ has been "cut" from (SM.9). Thus, inference targeting (SM.10) allows for a joint estimate of $\boldsymbol{\alpha}$ and $\boldsymbol{\theta}$ in which there is no chance of unwanted feedback from $\boldsymbol{y}$ influencing $\boldsymbol{\theta}$. Furthermore, uncertainty in the interference structure can still be propagated to $\boldsymbol{\alpha}$ by

marginalizing over $\boldsymbol{\theta}$ in (SM.10). For convenience, we will hereafter refer to all estimates targeting (SM.10) which marginalize over uncertainty in the interference structure as coming from **the cut feedback approach**. We obtain samples from (SM.10) using Algorithm 1.

**Algorithm 2** The Plug-In Approach

Fit the sulfate model, $\pi(\boldsymbol{\theta}|\bar{\boldsymbol{\eta}})$. ▷ *Posterior distribution of* $\boldsymbol{\theta}$ *when* $\bar{\boldsymbol{\eta}}$ *is observed but* $\boldsymbol{y}$ *is not.*
Calculate point estimate, $\hat{\boldsymbol{\theta}} = E(\boldsymbol{\theta}|\bar{\boldsymbol{\eta}})$.
Sample from $\pi(\boldsymbol{\alpha}|\boldsymbol{y}, \hat{\boldsymbol{\theta}})$. ▷ $\hat{\boldsymbol{\theta}}$ *is plugged into the outcome model.*

A second approach to modular inference is to disregard the propagation of uncertainty entirely. Instead, a point estimate, $\hat{\boldsymbol{\theta}}$, is estimated from the first module, and $\hat{\boldsymbol{\theta}}$ is then plugged into the second module, $\pi(\boldsymbol{\alpha} \mid \boldsymbol{y}, \hat{\boldsymbol{\theta}})$. This has been called the **plug-in** (or sometimes the *two-step*) **approach** [15, 23]. Notably, uncertainty in $\boldsymbol{\theta}$ has been sacrificed for the sake of computational convenience. In some ways, the plug-in approach mirrors previous attempts to estimate causal effects from observational studies with network interference. Namely, the interference structure (e.g., the network topology) is assumed to be fixed *a priori*, and any uncertainty about the network structure is ignored in the estimation of causal effects [1, 10, 27]. However, in the context of air pollution regulatory interventions, there is inherent uncertainty in the pollution transport process, and the propagation of this uncertainty (via the cutting feedback approach) may have a substantial impact on the associated causal effect estimates. Posterior samples with the plug-in approach are obtained using Algorithm 2.

### 5.2 Including Uncertainty in $G$: A Simulation Study

We performed a simulation study to investigate the differences in causal effect estimation under the cut feedback vs. plug-in approaches. The simulation study was conducted as follows. First, using the data and model described in Section 4 of the main paper, the pollution transport parameters are sampled from the fitted sulfate model posterior, i.e., $\boldsymbol{\theta}^{(k)} \sim \hat{\pi}(\boldsymbol{\theta} \mid \bar{\boldsymbol{\eta}})$. Using $\boldsymbol{\theta}^{(k)}$, the resulting interference network, $T^{(k)}$, and upwind exposure levels, $g_i^{(k)} = g_i(\boldsymbol{s}, T^{(k)})$ are calculated as described in Section 4 of the primary text. Then, outcome data, $\boldsymbol{y}^{(k)}$, are simulated from a data generating model, conditional on $\boldsymbol{x}_i$, $z_i$, and $g_i^{(k)}$. Note that $\boldsymbol{x}_i$ are a subset of the *observed* (i.e., not simulated) covariates used in the full analysis. Thus, the uncertainty in the simulated data comes from two sources: 1) the form of interference, as simulated from the posterior of the mechanistic model, which in turn dictates randomness in the neighborhood treatment, $g$, and 2) randomness in the outcomes, conditional on the treatments and covariates.

For each $\boldsymbol{y}^{(k)}$, we estimate the direct and indirect causal effects, $DE(g)$ and $IE(z, g)$, respectively, using four approaches: (i) a parametric outcome model (e.g., Poisson regression) with the plug-in approach, (ii) a parametric outcome model with the cut feedback approach, (iii) a nonparametric outcome model (e.g., log-linear BART regression) with plug-in, and (iv) a nonparametric outcome model with cut feedback. We note that the estimates are obtained using the same fitted process posterior, $\hat{\pi}(\boldsymbol{\theta}|\bar{\boldsymbol{\eta}})$, that was estimated from the observed sulfate data; the causal estimates are obtained by refitting the outcome model to the simulated data. This allows our simulation study to focus entirely on variation in causal estimates attributed to the choice of outcome model and the form of Bayesian modular inference. The simulations are repeated 100 times, and we compare the bias and 95% credible interval coverage rates of the four estimators for six values of $g$: $\{0.3, 0.4, 0.5, 0.6, 0.7, 0.8\}$. Finally, using Rubin's multiple imputation combining rules [21], we com-

pare the proportion of variance attributable to uncertainty in the interference structure for the cut feedback estimators.

**Data Generating Models**

**A. Gaussian Outcomes** $Y_i \sim Normal(\mu_i, \sigma^2 = 1)$

**CM1:** $\mu_i = \mathbf{x}_i'\beta - 1.2z_i - 0.4g_i - 1.7z_ig_i\,, \quad \beta = (2.5,1.6,\text{-}2.3,0.8,\text{-}1.1,\text{-}1.5,\text{-}0.5)'.$

**CM2:** $\mu_i = \begin{cases} \exp\{(\mathbf{x}_i - 0.5g_i\mathbf{1})'\beta\}, & z_i = 0 \\ \mathbf{x}_i'\beta - g_i^2, & z_i = 1 \end{cases}, \quad \beta = (\text{-}0.3,0.3,\text{-}0.3,\text{-}0.3,0.2,\text{-}0.4,0.6)'.$

**CM3:** $\mu_i = \begin{cases} \mathbf{x}_i'\beta_1 + z_i\mathbf{x}_i'\beta_2 - 0.3z_i + 1.7\,\mathbf{1}_{\{g_i<0.4\}}, & g_i < 0.65 \\ \exp\{-\mathbf{x}_i'\beta_1\} - 0.25z_i - (1+z_i)\sin\{40(g_i - 0.7)\}, & 0.65 \le g_i < 0.75, \\ \mathbf{x}_i'\beta_1 - 0.5z_i - 0.5\exp\{2g_i\}, & g_i \ge 0.75 \end{cases}$

$\beta_1 = (0.2,\text{-}0.1,1.3,\text{-}1.1,2.3,1.3,0.9)'$ and $\beta_2 = (\text{-}1.5,\text{-}0.7,\text{-}0.3,0.4,\text{-}0.5,2.0,1.0)'.$

**B. Poisson Outcomes**

$$Y_i \sim Poisson(\mu_{0i}\lambda_i), \quad \mu_{0i} = \textit{population size}$$

**PM1:** $\log\lambda_i = \mathbf{x}_i'\beta - 0.25z_i - 1.25g_i\,, \quad \beta = (\text{-}5.25,0.2,\text{-}0.2,0.1,0.15,\text{-}0.05,\text{-}0.15)'.$

**PM2:**
$$\log\lambda_i = 0.75 + \frac{1.5}{1+e^{-5x_{1i}}} - 0.5x_{2i} + 0.05x_{3i} + 4x_{4i}^2 + 2x_{4i} - \exp(-x_{5i}/25)$$
$$+0.1x_{6i} - 0.25z_i - 1.5z_ix_{1i} - 0.5g_i - 0.75g_ix_{1i}x_{2i}$$

**PM3:** $\log\lambda_i = \begin{cases} \mathbf{x}_i'\beta - 0.3z_i + 1.7\,\mathbf{1}_{\{g_i<0.4\}}, & g_i < 0.65 \\ \exp\{-\mathbf{x}_i'\beta\} - 0.25z_i - 0.1(1+z_i)\sin\{40(g_i - 0.7)\}, & 0.65 \le g_i < 0.75, \\ \mathbf{x}_i'\beta - 0.5z_i - 0.5\exp\{2g_i\}, & g_i \ge 0.75 \end{cases}$

$\beta = (\text{-}4.95,\text{-}0.025,0.325,\text{-}0.275,0.575,0.325,0.225)'.$

**Figure 12:** The data generating models used in the simulation studies, including (A) three continuous outcome models (CM1, CM2, CM3), and (B) three count (Poisson) outcome models (PM1, PM2, PM3).

We repeat this simulation study using six data generating models for $\boldsymbol{y}^{(k)}$, each simulating data from a different data generating model. The data generating models are shown in Figure 12: they include three continuous outcome models (CM1, CM2, and CM3), and three count (i.e., Poisson) outcome models (PM1, PM2, and PM3). The mean structures of the data generating models become increasingly complex — the increasing complexity is intended to compare the performance of parametric (e.g., linear regression) and nonparametric (e.g., BART) estimators, as well as the plug-in and cut feedback modular inference strategies, under a variety of data generating scenarios.

For convenience, we have summarized the simulation study procedure in Algorithm 3. The following notation is used in Algorithm 3 and when describing the results:

- $\hat{\pi}(\boldsymbol{\theta}|\bar{\boldsymbol{\eta}})$ denotes the fitted sulfate model (as described in Section 4.1 of the manuscript).
- $g_i^{(s)} = g_i(\boldsymbol{S}_{-j^*_{(i)}}, T(\boldsymbol{\theta}^{(s)}))$ denotes the upwind treatment exposure level, as determined by the bipartite network adjacency matrix, $T(\boldsymbol{\theta})$, and $\boldsymbol{S}_{-j^*_{(i)}}$, the vector of power plant treatments at all non-key-associated facilities.
- $\bar{\boldsymbol{g}}$ = estimated upwind exposure levels using $\bar{\boldsymbol{\theta}} = \hat{E}(\boldsymbol{\theta}|\bar{\boldsymbol{\eta}})$.
- $\boldsymbol{X}$ = a covariate matrix, consisting of an intercept and six covariates:
  - $x_0$ = intercept
  - $x_1$ = the proportion of black residents
  - $x_2$ = log(median income)
  - $x_3$ = log(population density)
  - $x_4$ = smoking rate
  - $x_5$ = annual precipitation total
  - $x_6$ = log(operating time) (of the key-associated power plant)

  For convenience, the covariates have been standardized to have mean zero and unit variance.
- $\boldsymbol{X}$, $\boldsymbol{S}$, and $\boldsymbol{z}$ are the same across all simulations; they were obtained from the data used in our full analysis (i.e., they were not simulated).

**Algorithm 3** Simulation Study

**for** $s = 1,\ldots, n_{sim}$ **do**

  Sample $\boldsymbol{\theta}^{(s)} \sim \hat{\pi}(\boldsymbol{\theta}|\bar{\boldsymbol{\eta}})$ ▷ Draw $\boldsymbol{\theta}$ from estimated sulfate model posterior.

  Calculate $g_i^{(s)} = g_i(\boldsymbol{S}_{-j^*_{(i)}}, T(\boldsymbol{\theta}^{(s)}))$ ▷ Upwind exposure level.

  Simulate $\boldsymbol{y}^{(s)} \sim \texttt{Outcome}(\boldsymbol{X}, \boldsymbol{z}, \boldsymbol{g}^{(s)})$ ▷ Simulate outcomes.

  **procedure** PLUG-IN($\boldsymbol{y}^{(s)}$, $\boldsymbol{X}$, $\boldsymbol{z}$, $\bar{\boldsymbol{g}}$) ▷ No uncertainty in $\boldsymbol{g}$.

    Estimate $E(\boldsymbol{y}^{(s)}|\boldsymbol{X}, \boldsymbol{z}, \bar{\boldsymbol{g}})$ using:

      $\pi_P(\boldsymbol{\alpha}|\boldsymbol{y}^{(s)}, \boldsymbol{X}, \boldsymbol{z}, \bar{\boldsymbol{g}}) \leftarrow$ Bayesian Linear Regression

      $\pi_{NP}(\boldsymbol{\alpha}|\boldsymbol{y}^{(s)}, \boldsymbol{X}, \boldsymbol{z}, \bar{\boldsymbol{g}}) \leftarrow$ Bayesian Nonparametric Regression (i.e., BART)

    Estimate $DE(g)$, $IE(z, g)$ using $\pi_P$ and $\pi_{NP}$.

  **end procedure**

  **procedure** CUT FEEDBACK($\boldsymbol{y}^{(s)}$, $\boldsymbol{X}$, $\boldsymbol{z}$, $\pi(\boldsymbol{\theta}|\bar{\boldsymbol{\eta}})$) ▷ Propagate uncertainty in $\boldsymbol{g}$.

    **for** $k = 1,\ldots,K$ **do**

      Sample $\boldsymbol{\theta}^{(k)} \sim \hat{\pi}(\boldsymbol{\theta}|\bar{\boldsymbol{\eta}})$

      Calculate $g_i^{(sk)} = g_i(\boldsymbol{S}_{-j^*_{(i)}}, T(\boldsymbol{\theta}^{(k)}))$

      Estimate $E(\boldsymbol{y}^{(s)}|\boldsymbol{X}, \boldsymbol{z}, \boldsymbol{g}^{(sk)})$ using:

        $\pi_P(\boldsymbol{\alpha}|\boldsymbol{y}^{(s)}, \boldsymbol{X}, \boldsymbol{z}, \boldsymbol{g}^{(sk)}) \leftarrow$ Bayesian Linear Regression

        $\pi_{NP}(\boldsymbol{\alpha}|\boldsymbol{y}^{(s)}, \boldsymbol{X}, \boldsymbol{z}, \boldsymbol{g}^{(sk)}) \leftarrow$ Bayesian Nonparametric Regression (e.g., BART)

      Estimate $DE(g)^{(sk)}$, $IE(z, g)^{(sk)}$ using $\pi_P$ and $\pi_{NP}$.

    **end for**

    Pool $DE(g)^{(sk)}$, $IE(z, g)^{(sk)}$ for $k = 1, \ldots, K$

  **end procedure**

  Compare $DE(g)$ and $IE(z, g)$ estimates from the Plug-In and Cut Feedback procedures

    $\rightarrow$ Includes parametric and nonparametric estimates

**end for**

## 5.3 Simulation Study Results

### 5.3.1 Estimating Bias, Coverage, and Proportion of Variance

We simulate 100 data sets from each data generating model (Figure 12). For each simulated data set, we estimate the direct effects, $DE(g)$, and indirect effects, $IE(z, g)$, for six values of $g$ ($g \in \{0.3, 0.4, 0.5, 0.6, 0.7, 0.8\}$); these effects are estimated using four approaches:

1. a parametric outcome model (e.g., Poisson or linear regression) using the plug-in approach (Algorithm 2),
2. a parametric outcome model using the cut feedback approach (Algorithm 1),
3. a nonparametric outcome model (e.g., BART/log-linear BART) using the plug-in approach,
4. a nonparametric outcome model using the cut feedback approach.

The four competing estimators are compared, with a focus on the bias and 95% credible interval coverage properties of the marginal effect estimates. For a population parameter $\gamma_0$, these are estimated as

$$Bias(\hat{\gamma}, \gamma) = E(\hat{\gamma}) - \gamma_0 = \frac{1}{n_{sim}} \sum_{k=1}^{n_{sim}} \hat{\gamma}^{(k)} - \gamma_0 \tag{SM.11}$$

and

$$\hat{C}_{\hat{\gamma}} = \frac{1}{n_{sim}} \sum_{k=1}^{n_{sim}} \mathbb{1}_{\{0.025 \leq \hat{p}_k \leq 0.975\}}, \tag{SM.12}$$

where

$$\hat{p}_k = \hat{Pr}(\gamma^{(k)} < \gamma_0 \,|\, \cdot) = \hat{F}_k(\gamma_0) \tag{SM.13}$$

denotes the empirical distribution function of the $k$th simulation, evaluated for $\gamma_0$. Thus, $\hat{C}_{\hat{\gamma}}$ is an estimate of the expected 95% credible interval coverage rate for an estimator, $\hat{\gamma}$.

Lastly, given the similarity of the cut feedback approach to multiple imputation, we co-opt Rubin's combining rules for multiple imputation [21, 18] to quantify the total variance of an estimator as a sum of the outcome model variance (i.e., the "within" variance) and the interference model variance (i.e., the "between" variance). Let $Q$ denote the population-level parameter of interest, such as $DE(g)$. Then, $\bar{Q} = \frac{1}{K}\sum_{i=1}^{K} \hat{Q}_i$ denotes the cut feedback point estimate of $Q$, where $\hat{Q}_i$ is the posterior mean estimate of $Q$ using the $i$th draw of $\boldsymbol{\theta} \sim \hat{\pi}(\boldsymbol{\theta}|\boldsymbol{\eta})$. In other words, this is the estimate of $DE(g)$ with the outcome model fitted conditional on $\boldsymbol{\theta}^{(k)}$. Then, the total variance of $\bar{Q}$ can be partitioned as,

$$Var(\bar{Q}) = \bar{U} + (1 + \frac{1}{K})B, \tag{SM.14}$$

where

$$\bar{U} = \frac{1}{K} \sum_{i=1}^{K} Var(\hat{Q}_i) \quad (\textit{within} \text{ cut variance}) \tag{SM.15}$$

and

$$B = \frac{1}{K-1} \sum_{i=1}^{K} (\hat{Q}_i - \bar{Q})^2 \quad (\textit{between} \text{ cut variance}). \tag{SM.16}$$

Thus, $\bar{U}$ represents the variance of $\bar{Q}$ due to uncertainty in the outcome model, while $B$ represents the variance of $\bar{Q}$ due to uncertainty in the interference structure. The inflation of $B$ in the calculation

of $Var(\bar{Q})$ is an adjustment proposed by Rubin [21] to account for the finite sample properties of the cut algorithm (Algorithm 1). The relative influence of the uncertainty due to interference can be summarized with

$$\rho_I = B/Var(\bar{Q}), \tag{SM.17}$$

the proportion of total variance attributed to the estimated interference structure. We estimate $\rho_I$ for the parametric and nonparametric cut feedback estimators in each simulation study.

### 5.3.2 Major Findings

The results from the six simulation studies are presented in detail in Sections 5.3.3–5.3.8. We summarize here the major findings, focusing on (a) the importance of propagating uncertainty in the estimated interference structure to the causal effect estimates, and (b) the comparative performance of causal effect estimation using log-linear BART against parametric alternatives.

First, consider data simulated from a simple outcome model (PM1):

$$Y_i^{(k)}|\boldsymbol{x}_i, z_i, g_i^{(k)} \overset{ind}{\sim} \text{Pois}(\mu_{0i}\lambda_i), \;\; i = 1, \ldots, n \tag{SM.18}$$

where

$$\log \lambda_i = \boldsymbol{x}_i'\boldsymbol{\beta} + \phi Z_i + \gamma G_i, \tag{SM.19}$$

$\mu_{0i}$ is a fixed offset denoting ZCTA $i$'s population size, $\phi = -0.25$, and $\gamma = 01.25$. When comparing bias, the plug-in and cut feedback estimators are comparable; the difference between the two approaches is instead most obvious when comparing coverage properties. For example, consider the 95% credible interval coverage rates of the estimators with Poisson outcome model (Figure 13). In this case, the plug-in estimator's coverage rates are well below 0.95 — for $DE(g)$, the rate starts at 0.5 for low $g$, steadily increasing to 0.9 as $g$ increases; for $IE(z, g)$, the rate is consistently around 0.3 for all values of $z$ and $g$. In contrast, the cut feedback estimator has coverage rates consistently around 0.95. In other words, when the outcome model is correctly specified, the plug-in estimator fails to propagate uncertainty from the estimated interference structure to the causal effect estimates, resulting in credible intervals that are too narrow. The cut feedback estimator accounts for uncertainty in the interference structure, which is reflected in the credible interval coverage rates.

The comparison between the log-linear BART and Poisson estimators is also of interest. In this simulation study, the Poisson estimators have lower bias than log-linear BART, a consequence of the correctly specified Poisson outcome model compared to the more general, nonparametric log-linear BART model. Furthermore, the log-linear BART estimator is inherently more conservative (a consequence of the nonparametric model's flexibility), and coverage rates for the plug-in and cut feedback approaches are very high — at or near 1 for $DE(g)$ and $IE(z, g)$ (Figure 13). Finally, we calculate the proportion of variance attributed to uncertainty in the interference structure (Figure 13 B). We see that the majority of the (correctly specified) Poisson cut feedback estimator's variance is attributed to uncertainty in the interference structure. In contrast, the BART estimator's variance is largely attributed to variance in the outcome model.

To further assess the performance of the log-linear BART estimator, we performed additional simulation studies with increasingly complex rate functions. For example, in PM3, $\log \lambda_i$ is highly nonlinear, with piecewise functions for three different segments of $g \in [0, 1]$ and complex interactions involving functions of $z_i$ and $g_i$. Once again, we found that conditional on the choice of outcome

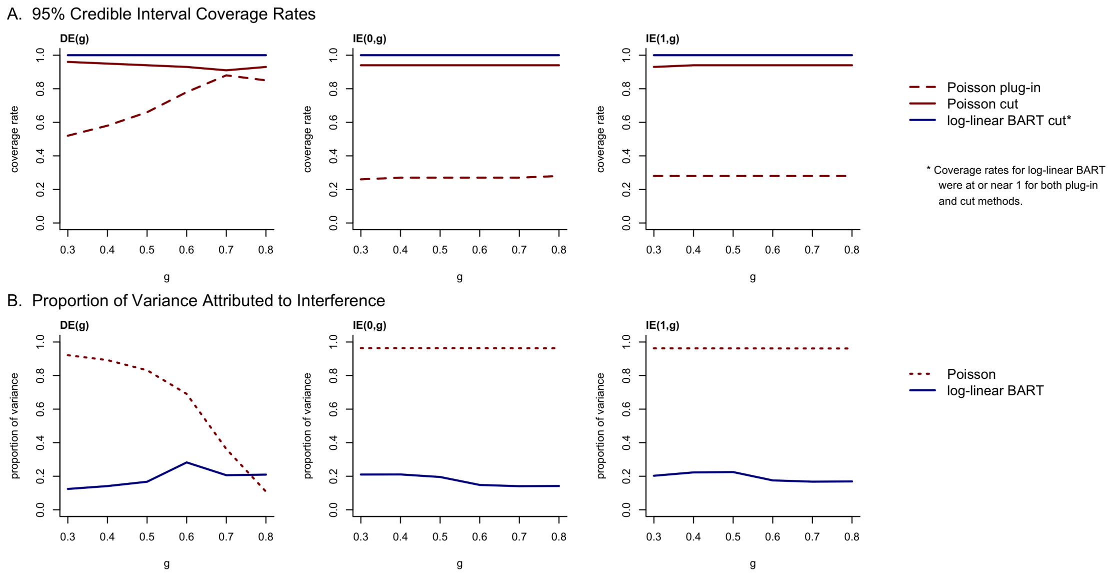


**Figure 13:** Results from PM1, including (A) 95% credible interval coverage rates and (B) proportion of variance attributed to the interference structure for four different estimators.

model, the plug-in and cut feedback estimators exhibited similar levels of bias. However, as the nonlinearity of $\log \lambda_i$ increases, the log-linear BART estimators exhibit *smaller* bias than the Poisson outcome model estimators. In other words, log-linear BART is adept at fitting nonlinear response surfaces [19], while parametric response surface models prove susceptible to model misspecification. The corresponding 95% credible interval coverage rates for all estimators are lower for simulations from PM3 than observed with PM1 (Figure 14). However, we find that 1) the cut feedback estimators have higher coverage rates than plug-in estimators, and 2) in general, the coverage rates for $DE(g)$ estimators with log-linear BART are higher than with Poisson outcome models; the coverage rates for $IE(z, g)$ are more variable. Finally, the proportion of variance attributed to uncertainty in the interference structure is highest for Poisson estimators (often near one, see Figure 14B).

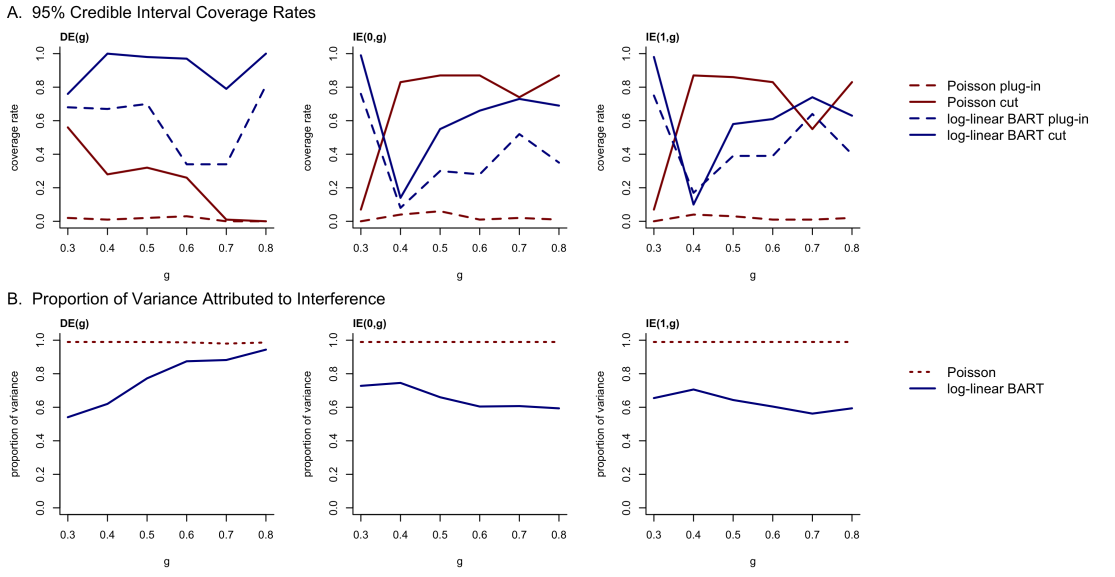


**Figure 14:** Results from PM3 with nonlinear $\log \lambda_i$, including (A) 95% credible interval coverage rates and (B) proportion of variance attributed to the interference structure for four different estimators.

Across all simulations, we found that large values of $\rho_I$ (the proportion of variance attributed to uncertainty in the interference structure) were associated with substantial improvement in coverage properties when using cut feedback estimates over the plug-in alternatives; at the very least, $\rho_I$ serves as an indicator that uncertainty in the interference structure should not be overlooked when making causal claims. To illustrate this phenomenon, we compared $\Delta\hat{C}_\gamma = \hat{C}_{\gamma_{\text{cut}}} - \hat{C}_{\gamma_{\text{plug-in}}}$, the observed difference between the cut feedback and plug-in 95% credible interval coverage rates for a population parameter, $\gamma$. For each simulation study, we calculated $\Delta\hat{C}_{DE(g)}$, $\Delta\hat{C}_{IE(0,g)}$, and $\Delta\hat{C}_{IE(1,g)}$ for the parametric (i.e., Poisson or linear regression) and nonparametric (e.g., BART/log-linear BART) estimators; this was done for six marginal values of $g$ ($g = 0.3, 0.4, 0.5, 0.6, 0.7, 0.8$). Then, each estimate of $\Delta\hat{C}$ was compared with the corresponding $\rho_I$ calculated from the cut feedback estimates, for a total of 252 $(\rho_I, \Delta\hat{C})$ pairs. As shown in Figure 15, we see a positive correlation ($r = 0.78$) between $\rho_I$ and $\Delta\hat{C}$; this is true when partitioning by type of estimator (parametric vs. nonparametric) or type of estimand (i.e., $DE(g)$, $IE(0, g)$, and $IE(1, g)$). Consequently, we advise practitioners to calculate and report $\rho_I$ when using the cut feedback approach, and to consider increasing the number of $\boldsymbol{\theta}$ samples if $\rho_I$ is close to one.

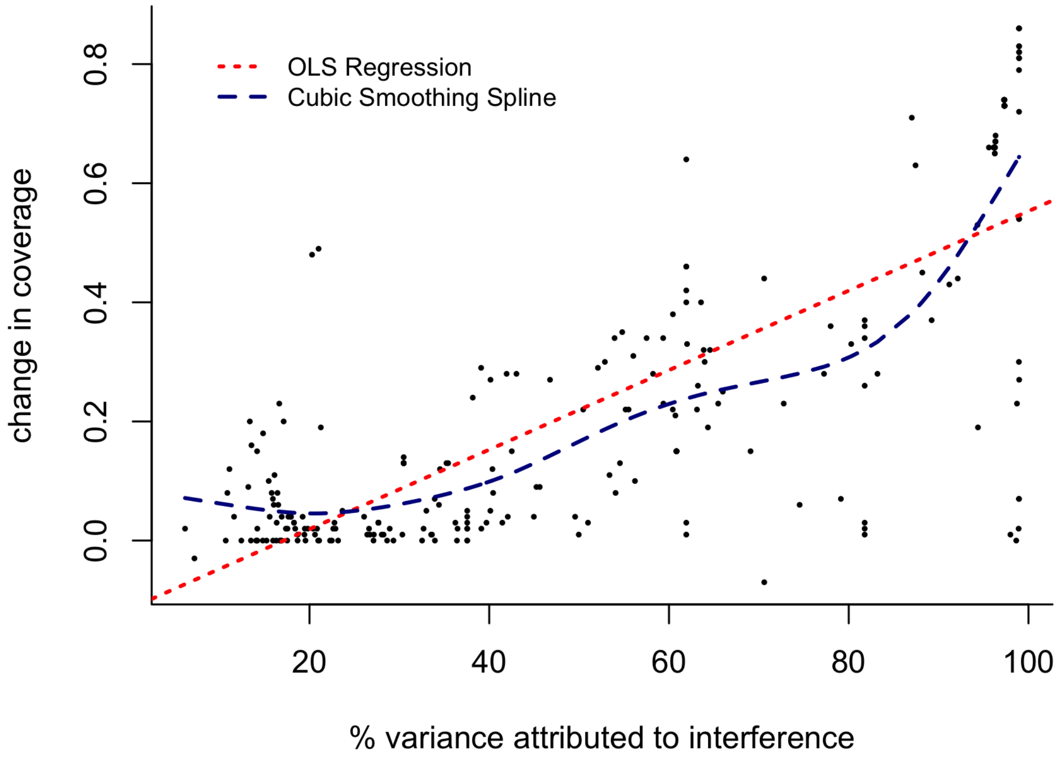


**Figure 15:** A comparison of the change in coverage between the plug-in and cut feed back estimators vs. the percent of variance attributable to uncertainty in the interference structure.

In summary, although the plug-in and cut feedback estimators exhibit similar levels of bias, their coverage properties often differ — the plug-in estimator's coverage rates are almost always lower than the corresponding cut estimator. The failure to propagate uncertainty from the interference

model to the effect estimates is most pronounced when fitting a parametric response surface model, when uncertainty in the interference structure dominates (as in PM1, for example). In contrast, the flexibility of log-linear BART comes with a cost: conservative uncertainty quantification, with a larger proportion of the total variance attributed to uncertainty in the outcome model. However, log-linear BART proves adept at estimating increasingly nonlinear dose-response surfaces. Consequently, we advocate for future analyses to consider the cut feedback approach to modular inference, given its ability to propagate (and quantify the proportion of) uncertainty from the estimated interference structure to the causal effect estimates. Furthermore, results should include a nuanced discussion of the choice of outcome model and its contribution to the total variance of the reported causal effect estimates. For a discussion of results from individual simulation studies, see Sections 5.3.3–5.3.8.

### 5.3.3 Results: CM1

Data were simulated from the following outcome model (CM1):

$$Y_i|\mu_i \overset{ind}{\sim} \text{Gaussian}(\mu_i, \sigma^2), \tag{SM.20}$$

$$\mu_i = \boldsymbol{x}_i'\boldsymbol{\beta} - 1.2z_i - 0.4g_i - 1.7z_ig_i, \tag{SM.21}$$

where $\boldsymbol{\beta} = (2.5, 1.6, -2.3, 0.8, -1.1, -1.5, -0.5)'$ and $\sigma^2 = 1$. Estimates of $DE(g)$ and $IE(z,g)$ were calculated for $z \in \{0,1\}$ and $g \in \{0.3, 0.4, 0.5, 0.6, 0.7, 0.8\}$, using four different estimation strategies: 1. Bayesian linear regression (with $z * g$ interaction) using the plug-in approach (LM plug-in), 2. Bayesian linear regression using the cut feedback approach (LM cut), 3. BART plug-in, and 4. BART cut. Estimated $DE(g)$ and $IE(z,g)$ curves from an example simulation are shown in Figures 16, 17, and 18.

The results from 100 simulations of CM1 are shown in Table SM.3. Unsurprisingly, estimates of $DE(g)$, $IE(0,g)$, and $IE(1,g)$ obtained from the linear regression model (i.e., the "true" model) have smaller bias than estimates obtained with BART regression. This is true for all marginal values of $g$ considered in the study. In addition, we see that when using either linear and BART regression, the difference in bias between the plug-in and cut feedback estimates is minimal. Instead, the strength of the cut feedback approach is most apparent when comparing the coverage properties of the linear regression model under the plug-in vs. cut feedback approaches. Notice that the LM plug-in estimates are slightly under-covered, especially for $IE(1,g)$; the coverage probabilities are closer to the expected 95% credible interval coverage rates when using LM cut. When comparing the BART results, we again see larger coverage probabilities when using the cut feedback strategy, however, in general the BART credible intervals are inherently conservative, and consequently the coverage probabilities are inflated when compared with their LM alternatives. The difference in uncertainty quantification is also visible in Figures 16, 17, and 18.

**Table SM.3:** Simulation study results (CM1).

| | Bias | | | Coverage | | |
|---|---|---|---|---|---|---|
| Method | DE($g$) | IE(0, $g$) | IE(1, $g$) | DE($g$) | IE(0, $g$) | IE(1, $g$) |
| $g = 0.3$ | | | | | | |
| LM plug-in | -0.039 | 0.001 | 0.007 | 0.94 | 0.93 | 0.80 |
| LM cut | -0.014 | -0.003 | -0.003 | 0.98 | 0.96 | 0.95 |
| BART plug-in | -0.359 | -0.014 | 0.065 | 0.87 | 0.99 | 0.99 |
| BART cut | -0.416 | 0.002 | 0.082 | 0.95 | 1.00 | 1.00 |
| $g = 0.4$ | | | | | | |
| LM plug-in | -0.028 | 0.003 | 0.020 | 0.94 | 0.93 | 0.80 |
| LM cut | -0.014 | -0.009 | -0.008 | 0.99 | 0.96 | 0.95 |
| BART plug-in | -0.239 | -0.079 | 0.119 | 0.92 | 0.99 | 0.98 |
| BART cut | -0.277 | -0.028 | 0.190 | 0.98 | 1.00 | 1.00 |
| $g = 0.5$ | | | | | | |
| LM plug-in | -0.017 | 0.005 | 0.033 | 0.95 | 0.93 | 0.80 |
| LM cut | -0.013 | -0.016 | -0.013 | 0.99 | 0.96 | 0.95 |
| BART plug-in | -0.168 | -0.086 | 0.183 | 0.97 | 0.98 | 0.95 |
| BART cut | -0.167 | -0.072 | 0.256 | 1.00 | 1.00 | 0.98 |
| $g = 0.6$ | | | | | | |
| LM plug-in | -0.006 | 0.007 | 0.046 | 0.95 | 0.93 | 0.80 |
| LM cut | -0.012 | -0.022 | -0.019 | 0.99 | 0.96 | 0.95 |
| BART plug-in | -0.060 | -0.126 | 0.251 | 0.98 | 0.98 | 0.94 |
| BART cut | -0.067 | -0.149 | 0.280 | 1.00 | 1.00 | 0.98 |
| $g = 0.7$ | | | | | | |
| LM plug-in | 0.005 | 0.009 | 0.059 | 0.93 | 0.93 | 0.80 |
| LM cut | -0.011 | -0.028 | -0.024 | 0.95 | 0.96 | 0.95 |
| BART plug-in | 0.050 | -0.183 | 0.304 | 0.97 | 0.98 | 0.93 |
| BART cut | 0.037 | -0.209 | 0.323 | 1.00 | 1.00 | 0.97 |
| $g = 0.8$ | | | | | | |
| LM plug-in | 0.017 | 0.011 | 0.073 | 0.89 | 0.93 | 0.80 |
| LM cut | -0.010 | -0.034 | -0.029 | 0.94 | 0.96 | 0.95 |
| BART plug-in | 0.175 | -0.233 | 0.379 | 0.88 | 0.98 | 0.94 |
| BART cut | 0.167 | -0.239 | 0.423 | 0.98 | 1.00 | 0.97 |

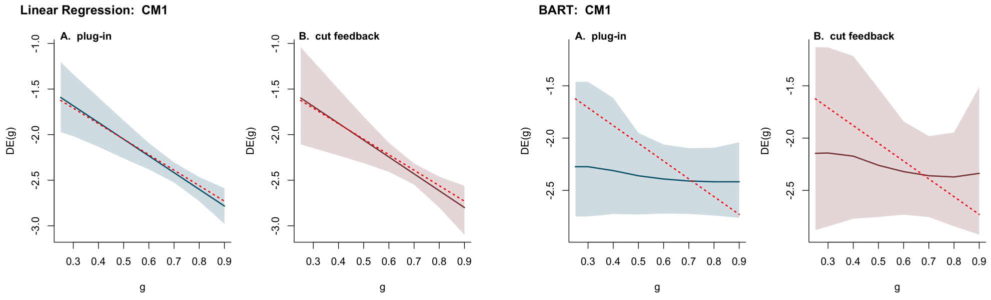


**Figure 16:** The estimated **direct effects** $(DE(g))$ for a simulation from CM1, using linear regression and BART regression, with a comparison between the plug-in and cut feedback approaches.

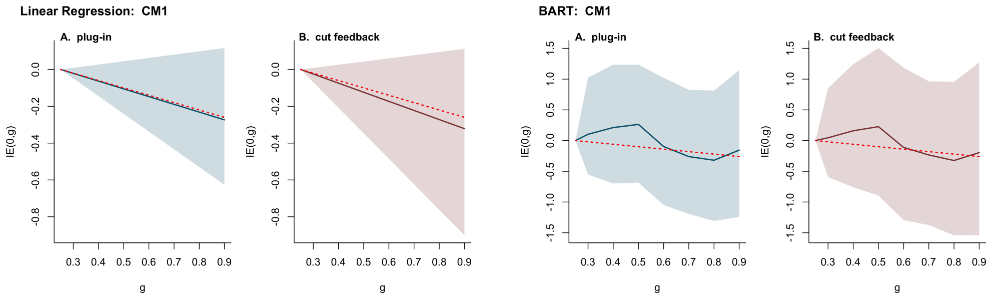


**Figure 17:** The estimated **indirect effects** $(IE(0, g))$ for a simulation from CM1, using linear regression and BART regression, with a comparison between the plug-in and cut feedback approaches.

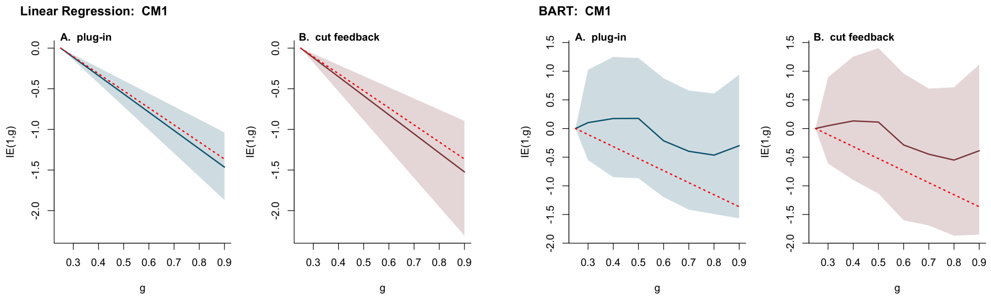


**Figure 18:** The estimated **indirect effects** $(IE(1, g))$ for a simulation from CM1, using linear regression and BART regression, with a comparison between the plug-in and cut feedback approaches.

#### 5.3.4 Results: CM2

Data were simulated from the following outcome model (CM2):

$$Y_i|\mu_i \overset{ind}{\sim} \text{Gaussian}(\mu_i, \sigma^2), \tag{SM.22}$$

$$\mu_i = \exp\{(\boldsymbol{x}_i' - 0.5g_i\mathbf{1})'\boldsymbol{\beta}\}\mathbb{1}_{\{z_i=0\}} + (\boldsymbol{x}_i'\boldsymbol{\beta} - g_i^2)\mathbb{1}_{\{z_i=1\}}, \tag{SM.23}$$

where $\boldsymbol{\beta} = (-0.3, 0.3, -0.3, -0.3, 0.2, -0.4, 0.6)'$ and $\sigma^2 = 1$. Notice that $\mu_i$ is no longer linear, but instead exhibits nonlinearities and interactions between $z_i$, $g_i$, and $\boldsymbol{x}_i$. The mean structure was chosen to mimic that found in the simulation studies in Jennifer Hill's paper detailing how BART may be used for causal inference (2011). Estimates of $DE(g)$ and $IE(z, g)$ were calculated for $z \in \{0, 1\}$ and $g \in \{0.3, 0.4, 0.5, 0.6, 0.7, 0.8\}$, using four different estimation strategies: 1. Bayesian linear regression (with $z * g$ interaction) using the plug-in approach (LM plug-in), 2. Bayesian linear regression using the cut feedback approach (LM cut), 3. BART plug-in, and 4. BART cut. Estimated $DE(g)$ and $IE(z, g)$ curves from an example simulation are shown in Figures 19, 20, and 21.

As shown in Table SM.4, the BART causal effect estimates are now competitive with the LM effect estimates (in terms of bias), especially when comparing the bias of estimates when $g$ is small (0.3, 0.4, 0.5) or large (0.8). Conversely, the LM estimates perform best for $g = 0.6$ and 0.7 — this corresponds to the regions of $\hat{F}(g)$ with the most mass. In other words, inference with BART may be preferable to linear regression when the dose-response surface is nonlinear, or if the covariate data are sparse. For both LM and BART, the plug-in and cut feedback estimators exhibit similar levels of bias. However, when comparing coverage properties, the cut feedback estimators have larger coverage probabilities than the plug-in estimators. Furthermore, the coverage of the LM estimators is often low, while the BART estimators remain conservative in their uncertainty quantification, resulting in high coverage properties.

**Table SM.4:** Simulation study results (CM2).

| | Bias | | | Coverage | | |
|---|---|---|---|---|---|---|
| Method | DE($g$) | IE(0, $g$) | IE(1, $g$) | DE($g$) | IE(0, $g$) | IE(1, $g$) |
| $g = 0.3$ | | | | | | |
| LM plug-in | -0.494 | -0.047 | -0.019 | 0.31 | 0.1 | 0.84 |
| LM cut | -0.496 | -0.053 | -0.026 | 0.54 | 0.25 | 0.84 |
| BART plug-in | -0.482 | -0.011 | 0.025 | 0.89 | 0.99 | 1.00 |
| BART cut | -0.478 | -0.018 | 0.014 | 0.97 | 1.00 | 1.00 |
| $g = 0.4$ | | | | | | |
| LM plug-in | -0.424 | -0.142 | -0.043 | 0.27 | 0.1 | 0.87 |
| LM cut | -0.427 | -0.160 | -0.064 | 0.43 | 0.25 | 0.89 |
| BART plug-in | -0.400 | -0.094 | 0.024 | 0.85 | 0.98 | 0.99 |
| BART cut | -0.406 | -0.039 | 0.066 | 0.97 | 1.00 | 1.00 |
| $g = 0.5$ | | | | | | |
| LM plug-in | -0.333 | -0.236 | -0.047 | 0.18 | 0.1 | 0.90 |
| LM cut | -0.338 | -0.266 | -0.082 | 0.30 | 0.25 | 0.90 |
| BART plug-in | -0.360 | 0.055 | 0.214 | 0.81 | 1.00 | 0.98 |
| BART cut | -0.347 | 0.016 | 0.179 | 0.96 | 1.00 | 1.00 |
| $g = 0.6$ | | | | | | |
| LM plug-in | -0.223 | -0.331 | -0.0319 | 0.16 | 0.1 | 0.94 |
| LM cut | -0.229 | -0.373 | -0.079 | 0.19 | 0.25 | 0.97 |
| BART plug-in | -0.294 | 0.010 | 0.234 | 0.80 | 0.99 | 0.94 |
| BART cut | -0.300 | 0.014 | 0.225 | 0.96 | 1.00 | 1.00 |
| $g = 0.7$ | | | | | | |
| LM plug-in | -0.092 | -0.425 | 0.005 | 0.67 | 0.1 | 0.95 |
| LM cut | -0.099 | -0.480 | -0.057 | 0.64 | 0.25 | 0.99 |
| BART plug-in | -0.155 | -0.122 | 0.241 | 0.93 | 0.98 | 0.96 |
| BART cut | -0.179 | -0.097 | 0.234 | 1.00 | 1.00 | 1.00 |
| $g = 0.8$ | | | | | | |
| LM plug-in | 0.059 | -0.520 | 0.061 | 0.88 | 0.1 | 0.96 |
| LM cut | 0.050 | -0.587 | -0.014 | 0.93 | 0.25 | 0.98 |
| BART plug-in | -0.014 | -0.222 | 0.282 | 0.99 | 0.96 | 0.96 |
| BART cut | -0.047 | -0.178 | 0.285 | 1.00 | 1.00 | 1.00 |

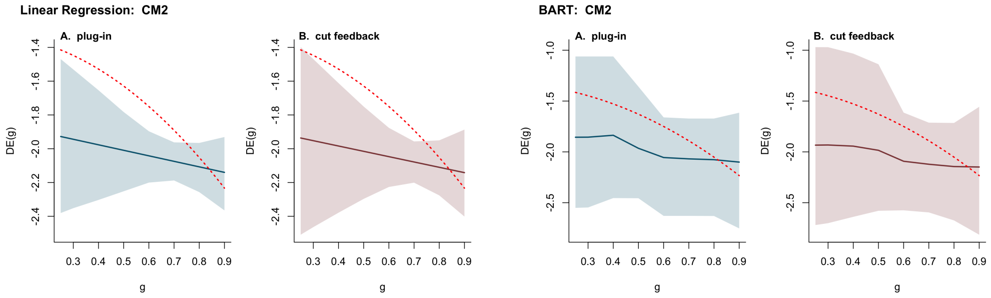


**Figure 19:** The estimated **direct effects** $(DE(g))$ for a simulation from CM2, using linear regression and BART regression, with a comparison between the plug-in and cut feedback approaches.

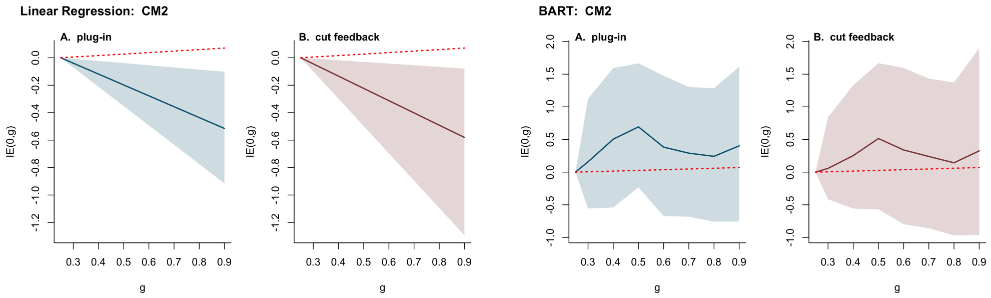


**Figure 20:** The estimated **indirect effects** $(IE(0, g))$ for a simulation from CM2, using linear regression and BART regression, with a comparison between the plug-in and cut feedback approaches.

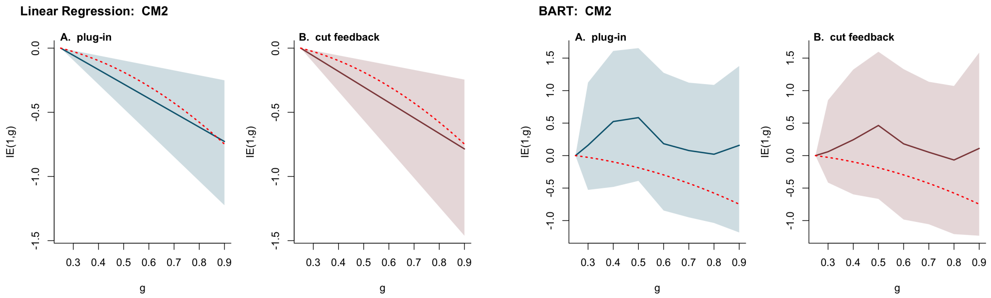


**Figure 21:** The estimated **indirect effects** $(IE(1, g))$ for a simulation from CM2, using linear regression and BART regression, with a comparison between the plug-in and cut feedback approaches.

#### 5.3.5 Results: CM3

Data were simulated from the following outcome model (CM2):

$$Y_i|\mu_i \overset{ind}{\sim} \text{Gaussian}(\mu_i, \sigma^2), \tag{SM.24}$$

$$\mu_i = \begin{cases} \boldsymbol{x}_i'\boldsymbol{\beta}_1 + z_i\boldsymbol{x}_i'\boldsymbol{\beta}_2 - 0.3z_i + 1.7\mathbb{1}_{\{g_i<0.4\}} & g_i < 0.65 \\ \exp\{-\boldsymbol{x}_i'\boldsymbol{\beta}_1\} - 0.25z_i + (1+z_i)\sin\{40(g_i - 0.7)\}, & 0.65 \le g_i < 0.75 \\ \boldsymbol{x}_i'\boldsymbol{\beta}_1 - 0.5z_i - 0.5\exp\{2g_i\}, & g_i \ge 0.75 \end{cases} \tag{SM.25}$$

where $\boldsymbol{\beta}_1 = (0.2, -0.1, 1.3, -1.1, 2.3, 1.3, 0.9)'$, $\boldsymbol{\beta}_2 = (-1.5, -0.7, -0.3, 0.4, -0.5, 2.0, 1.0)'$ and $\sigma^2 = 1$. Again, $\mu_i$ has been chosen to be very nonlinear, with corresponding nonlinear direct and indirect effect curves (e.g., the red curve in Figures 22). This was done to illustrate BART's nonlinearity. Estimates of $DE(g)$ and $IE(z, g)$ were calculated for $z \in \{0, 1\}$ and $g \in \{0.3, 0.4, 0.5, 0.6, 0.7, 0.8\}$, using four different estimation strategies: 1. Bayesian linear regression (with $z * g$ interaction) using the plug-in approach (LM plug-in), 2. Bayesian linear regression using the cut feedback approach (LM cut), 3. BART plug-in, and 4. BART cut. Estimated $DE(g)$ and $IE(z, g)$ curves from an example simulation are shown in Figures 22, 23, and 24.

In this study, the nonlinearity of BART is most advantageous — the BART estimates exhibit bias that is at least as small as the LM estimates, across the board. Furthermore, the BART cut feedback estimates of $DE(g)$ have smaller bias than the BART plug-in estimates (the estimates of $IE(z, g)$ are mostly equivalent). We again see that the cut feedback estimates have wider uncertainty bounds, on average, than the plug-in estimates. Consequently, the coverage probabilities are larger when using the cut estimators. In this study, both LM *and* BART are under-covered (LM much more so than BART). This is a consequence of model misspecification and a highly nonlinear $\mu_i$.

**Table SM.5:** Simulation study results (CM3).

| | Bias | | | Coverage | | |
|---|---|---|---|---|---|---|
| Method | DE($g$) | IE(0, $g$) | IE(1, $g$) | DE($g$) | IE(0, $g$) | IE(1, $g$) |
| $g = 0.3$ | | | | | | |
| LM plug-in | -2.927 | -0.579 | 0.010 | 0.20 | 0.00 | 0.75 |
| LM cut | -3.226 | -0.675 | -0.047 | 0.55 | 0.03 | 0.78 |
| BART plug-in | -0.984 | 0.016 | 0.047 | 0.72 | 1.00 | 1.00 |
| BART cut | -0.862 | -0.032 | -0.001 | 1.00 | 1.00 | 1.00 |
| $g = 0.4$ | | | | | | |
| LM plug-in | -1.748 | -0.038 | 1.731 | 0.75 | 0.97 | 0.00 |
| LM cut | -1.970 | -0.324 | 1.560 | 0.86 | 0.99 | 0.42 |
| BART plug-in | -0.929 | -0.164 | -0.077 | 0.70 | 0.96 | 0.96 |
| BART cut | -0.786 | -0.207 | -0.099 | 1.00 | 1.00 | 1.00 |
| $g = 0.5$ | | | | | | |
| LM plug-in | -0.569 | -1.197 | 1.751 | 0.91 | 0.11 | 0.11 |
| LM cut | -0.714 | -1.673 | 1.466 | 0.92 | 0.48 | 0.75 |
| BART plug-in | -0.795 | -0.748 | -0.528 | 0.67 | 0.71 | 0.86 |
| BART cut | -0.651 | -0.528 | -0.286 | 1.00 | 1.00 | 1.00 |
| $g = 0.6$ | | | | | | |
| LM plug-in | 0.610 | -2.356 | 1.771 | 0.55 | 0.01 | 0.49 |
| LM cut | 0.542 | -3.023 | 1.372 | 0.79 | 0.27 | 0.89 |
| BART plug-in | -0.451 | -0.207 | 0.358 | 0.66 | 0.83 | 0.82 |
| BART cut | -0.279 | -0.104 | 0.510 | 0.98 | 1.00 | 1.00 |
| $g = 0.7$ | | | | | | |
| LM plug-in | 0.239 | -8.336 | -4.579 | 0.69 | 0.00 | 0.03 |
| LM cut | 0.248 | -9.193 | -5.092 | 0.69 | 0.01 | 0.04 |
| BART plug-in | 2.530 | 2.378 | 5.924 | 0.03 | 0.45 | 0.01 |
| BART cut | 2.164 | 1.552 | 4.610 | 0.50 | 0.89 | 0.64 |
| $g = 0.8$ | | | | | | |
| LM plug-in | 1.669 | -2.197 | 2.989 | 0.13 | 0.28 | 0.42 |
| LM cut | 1.753 | -3.245 | 2.362 | 0.22 | 0.64 | 0.88 |
| BART plug-in | 1.239 | -2.881 | -0.626 | 0.37 | 0.21 | 0.55 |
| BART cut | 1.111 | -3.088 | -1.084 | 0.94 | 0.42 | 0.90 |

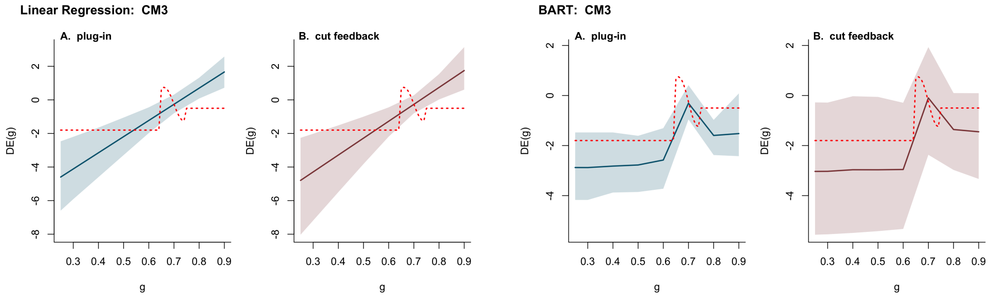


**Figure 22:** The estimated **direct effects** $(DE(g)$ for a simulation from CM3, using linear regression and BART regression, with a comparison between the plug-in and cut feedback approaches.

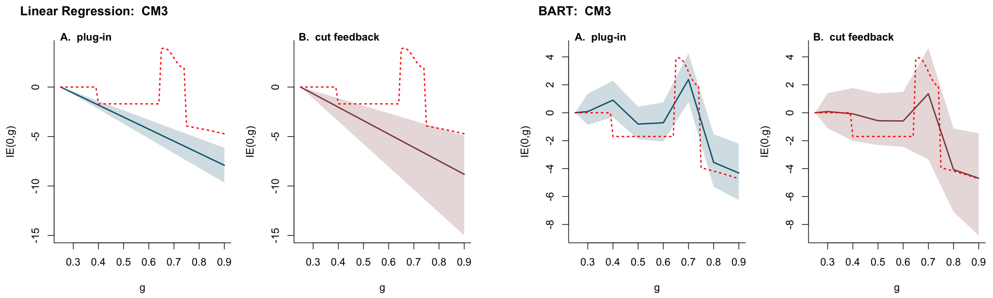


**Figure 23:** The estimated **indirect effects** $(IE(0, g))$ for a simulation from CM3, using linear regression and BART regression, with a comparison between the plug-in and cut feedback approaches.

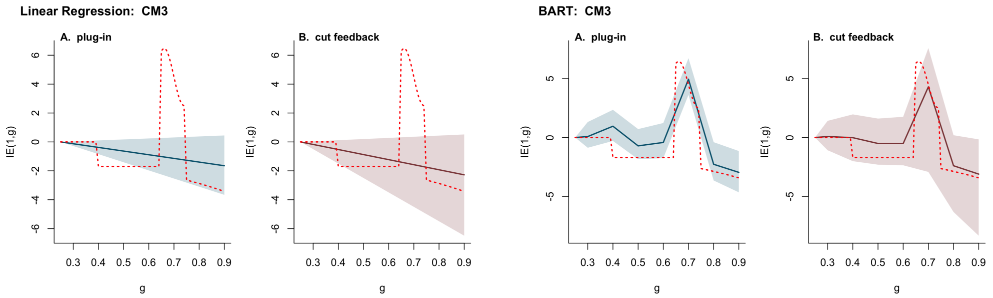


**Figure 24:** The estimated **indirect effects** $(IE(1, g))$ for a simulation from CM3, using linear regression and BART regression, with a comparison between the plug-in and cut feedback approaches.

#### 5.3.6 Results: PM1

Data were simulated from the following outcome model (PM1):

$$Y_i|\lambda_i \overset{ind}{\sim} \text{Poisson}(\mu_{0i}\lambda_i), \tag{SM.26}$$

$$\log \lambda_i = \boldsymbol{x}_i'\boldsymbol{\beta} - 0.25z_i - 1.25g_i, \tag{SM.27}$$

where $\boldsymbol{\beta} = (-5.25, 0.2, -0.2, 0.1, 0.15, -0.05, -0.15)'$ and $\mu_{0i}$ is an offset equal to the population size of ZCTA $i$. Similar to CM1, $\log \lambda_i$ has been chosen to have a simple linear structure, which will become more nonlinear with simulation studies PM2 and PM3. Estimates of $DE(g)$ and $IE(z, g)$ were calculated for $z \in \{0, 1\}$ and $g \in \{0.3, 0.4, 0.5, 0.6, 0.7, 0.8\}$, using four different estimation strategies: 1. Bayesian Poisson regression using the plug-in approach (Poisson plug-in), 2. Bayesian Poisson regression using the cut feedback approach (Poisson cut), 3. log-linear BART plug-in, and 4. log-linear BART cut. Estimated $DE(g)$ and $IE(z, g)$ curves from an example simulation are shown in Figures 25, 26, and 27.

The results from 100 simulation from PM1 are shown in Table SM.6. Unsurprisingly, estimates from the Poisson regression model (i.e., the "true" model) have smaller bias than estimates from log-linear BART. Furthermore, for both Poisson and BART regression, we see that the bias is approximately equivalent using either the plug-in or cut feedback estimation strategies. However, for Poisson regression, the cut feedback approach has desirable credible interval coverage properties compared to the plug-in approach. When using log-linear BART, the advantage of the cut feedback approach over the plug-in approach is less clear — log-linear BART's credible intervals are inherently conservative, and consequently the 95% credible interval coverage rates are near 1 regardless of method.

This becomes more apparent when comparing the estimated direct and indirect effects under Poisson and log-linear BART regression. The estimated direct effects are shown in Figure 25, while the estimated indirect effects are shown in Figures 26 and 27. Notice that the scale for the BART regression is much larger in magnitude than the scale for Poisson regression. Furthermore, the plug-in approach results in under coverage when using Poisson regression, while the uncertainty quantification with BART is large even when using the plug-in approach.

**Table SM.6:** Simulation study results (PM1).

| | Bias | | | Coverage | | |
|---|---|---|---|---|---|---|
| Method | DE($g$) | IE(0, $g$) | IE(1, $g$) | DE($g$) | IE(0, $g$) | IE(1, $g$) |
| $g = 0.3$ | | | | | | |
| Poisson plug-in | 0.040 | 0.025 | 0.019 | 0.50 | 0.28 | 0.33 |
| Poisson cut | -0.038 | -0.035 | -0.025 | 0.95 | 0.94 | 0.94 |
| BART plug-in | 0.597 | 0.240 | 0.182 | 1.00 | 0.51 | 0.52 |
| BART cut | 0.495 | 0.214 | 0.139 | 1.00 | 1.00 | 1.00 |
| $g = 0.4$ | | | | | | |
| Poisson plug-in | 0.029 | 0.068 | 0.052 | 0.51 | 0.28 | 0.33 |
| Poisson cut | -0.023 | -0.088 | -0.064 | 0.96 | 0.94 | 0.94 |
| BART plug-in | 0.339 | 0.276 | -0.041 | 1.00 | 1.00 | 1.00 |
| BART cut | 0.333 | 0.489 | 0.252 | 1.00 | 1.00 | 1.00 |
| $g = 0.5$ | | | | | | |
| Poisson plug-in | 0.021 | 0.106 | 0.081 | 0.57 | 0.28 | 0.33 |
| Poisson cut | -0.012 | -0.124 | -0.089 | 0.96 | 0.94 | 0.94 |
| BART plug-in | 0.164 | 0.360 | -0.131 | 1.00 | 1.00 | 1.00 |
| BART cut | 0.143 | 0.590 | 0.163 | 1.00 | 1.00 | 1.00 |
| $g = 0.6$ | | | | | | |
| Poisson plug-in | 0.013 | 0.138 | 0.105 | 0.74 | 0.28 | 0.33 |
| Poisson cut | -0.005 | -0.148 | -0.106 | 0.96 | 0.94 | 0.94 |
| BART plug-in | 0.068 | 0.433 | -0.154 | 0.98 | 1.00 | 1.00 |
| BART cut | 0.039 | 0.558 | 0.028 | 1.00 | 1.00 | 1.00 |
| $g = 0.7$ | | | | | | |
| Poisson plug-in | 0.006 | 0.164 | 0.125 | 0.84 | 0.28 | 0.33 |
| Poisson cut | -0.001 | -0.162 | -0.115 | 0.93 | 0.94 | 0.94 |
| BART plug-in | 0.050 | 0.474 | -0.131 | 0.97 | 0.99 | 1.00 |
| BART cut | 0.041 | 0.556 | 0.028 | 1.00 | 1.00 | 1.00 |
| $g = 0.8$ | | | | | | |
| Poisson plug-in | 0.001 | 0.186 | 0.142 | 0.90 | 0.28 | 0.33 |
| Poisson cut | 0.002 | -0.169 | -0.119 | 0.91 | 0.94 | 0.94 |
| BART plug-in | 0.039 | 0.521 | -0.096 | 1.00 | 0.98 | 1.00 |
| BART cut | 0.041 | 0.590 | 0.062 | 1.00 | 1.00 | 1.00 |

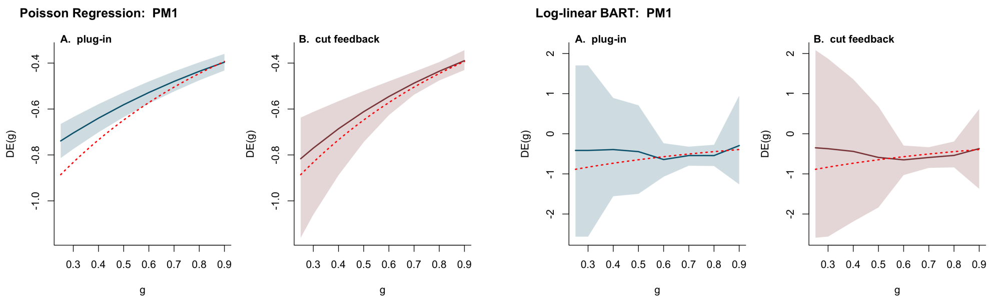


**Figure 25:** The estimated **direct effects** ($DE(g)$) for a simulation from PM1, using Poisson and log-linear BART regression, with a comparison between the plug-in and cutting feedback approaches.

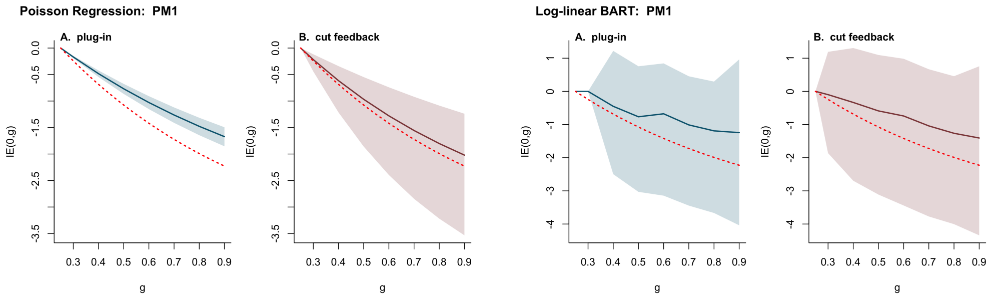


**Figure 26:** The estimated **indirect effects** ($IE(0, g)$) for a simulation from PM1, using Poisson and log-linear BART regression, with a comparison between the plug-in and cutting feedback approaches.

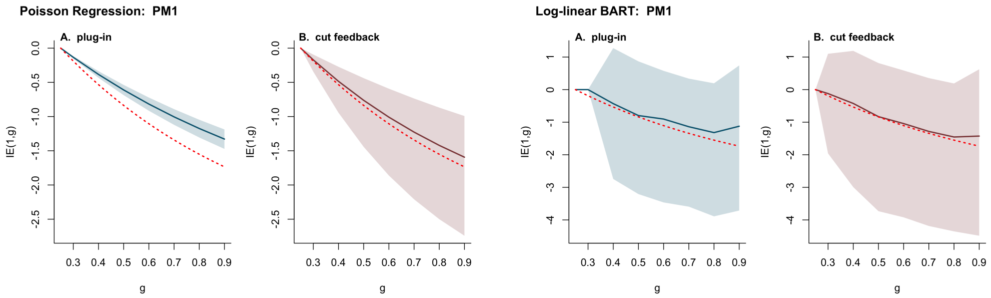


**Figure 27:** The estimated **indirect effects** ($IE(1, g)$) for a simulation from PM1, using Poisson and log-linear BART regression, with a comparison between the plug-in and cutting feedback approaches.

#### 5.3.7 Results: PM2

Data were simulated from the following outcome model (PM2):

$$Y_i|\lambda_i \overset{ind}{\sim} \text{Poisson}(\mu_{0i}\lambda_i), \tag{SM.28}$$

$$\begin{aligned} \log \lambda_i = 0.75 + &\frac{1.5}{1+e^{-5x_{1i}}} - 0.5x_{2i} + 0.05x_{3i} + 4x_{4i}^2 + 2x_{4i} \\ &- \exp(-x_{5i}/25) + 0.1x_{6i} - 0.25z_i - 1.5z_i x_{1i} - 0.5g_i - 0.75g_i x_{1i} x_{2i}, \end{aligned} \tag{SM.29}$$

with $\mu_{0i}$ denoting the offset equal to the population size of ZCTA $i$. Here, $\log \lambda_i$ has been chosen to have a nonlinear structure, including interactions between $z_i$, $g_i$, and covariates $x_1$ and $x_2$. Estimates of $DE(g)$ and $IE(z,g)$ were calculated for $z \in \{0,1\}$ and $g \in \{0.3, 0.4, 0.5, 0.6, 0.7, 0.8\}$, using four different estimation strategies: 1. Bayesian Poisson regression using the plug-in approach (Poisson plug-in), 2. Bayesian Poisson regression using the cut feedback approach (Poisson cut), 3. log-linear BART plug-in, and 4. log-linear BART cut. Estimated $DE(g)$ and $IE(z,g)$ curves from an example simulation are shown in Figures 28, 29, and 30.

The results of the simulation study are shown in Table SM.7. In general, we see that the log-linear BART $DE(g)$ estimates have lower bias than the Poisson regression estimates when $g \geq 0.5$ (i.e., the $g$ values with the most available data); when $g = 0.3$ or $0.4$, the log-linear BART prior shrinks the estimates back towards zero, resulting in larger bias. In contrast, the Poisson regression estimates of $IE(z,g)$ have lower bias than the corresponding log-linear BART estimates; this is likely due to the regularization-induced shrinking in the BART estimates for small $g$, which affect the estimates of $IE(z,g) = \mu(z,g) - \mu(z,g^*)$, where $g^* = 0.25$. When using either Poisson regression or log-linear BART, the bias of the plug-in and cut feedback estimates are very similar.

Once again, the 95% credible interval coverage rates are larger for cut feedback estimates when compared with the corresponding plug-in estimates. This is true when using either the Poisson regression and log-linear BART outcome models. Furthermore, the Poisson regression estimates are generally under-covered, especially for $DE(g)$. In contrast, the log-linear BART plug-ing estimates are slightly under-covered, while the cut feedback estimates are over-covered — this is likely due to log-linear BART's inherently conservative uncertainty quantification.

**Table SM.7:** Simulation study results (PM2).

| | Bias | | | Coverage | | |
|---|---|---|---|---|---|---|
| Method | DE($g$) | IE(0, $g$) | IE(1, $g$) | DE($g$) | IE(0, $g$) | IE(1, $g$) |
| $g = 0.3$ | | | | | | |
| Poisson plug-in | -0.031 | 0.150 | 0.095 | 0.31 | 0.20 | 0.21 |
| Poisson cut | -0.356 | 0.007 | 0.003 | 0.91 | 0.94 | 0.94 |
| BART plug-in | 1.086 | 1.280 | 0.801 | 0.98 | 0.72 | 0.73 |
| BART cut | 0.821 | 0.840 | 0.492 | 1.00 | 1.00 | 1.00 |
| $g = 0.4$ | | | | | | |
| Poisson plug-in | -0.133 | 0.432 | 0.276 | 0.37 | 0.20 | 0.21 |
| Poisson cut | -0.365 | 0.026 | 0.013 | 0.89 | 0.94 | 0.94 |
| BART plug-in | 0.640 | 1.612 | 0.686 | 0.98 | 0.98 | 1.00 |
| BART cut | 0.279 | 1.815 | 0.924 | 1.00 | 1.00 | 1.00 |
| $g = 0.5$ | | | | | | |
| Poisson plug-in | -0.226 | 0.691 | 0.442 | 0.36 | 0.20 | 0.21 |
| Poisson cut | -0.375 | 0.051 | 0.029 | 0.79 | 0.94 | 0.94 |
| BART plug-in | 0.218 | 2.034 | 0.686 | 0.95 | 0.94 | 1.00 |
| BART cut | 0.041 | 1.942 | 0.813 | 1.00 | 1.00 | 1.00 |
| $g = 0.6$ | | | | | | |
| Poisson plug-in | -0.311 | 0.930 | 0.595 | 0.18 | 0.20 | 0.21 |
| Poisson cut | -0.387 | 0.082 | 0.047 | 0.31 | 0.94 | 0.94 |
| BART plug-in | 0.077 | 2.363 | 0.875 | 0.96 | 0.94 | 1.00 |
| BART cut | -0.006 | 1.922 | 0.746 | 1.00 | 1.00 | 1.00 |
| $g = 0.7$ | | | | | | |
| Poisson plug-in | -0.389 | 1.149 | 0.737 | 0.00 | 0.20 | 0.22 |
| Poisson cut | -0.399 | 0.116 | 0.069 | 0.00 | 0.94 | 0.94 |
| BART plug-in | 0.081 | 2.434 | 0.950 | 0.98 | 0.90 | 0.99 |
| BART cut | 0.080 | 1.798 | 0.708 | 1.00 | 1.00 | 1.00 |
| $g = 0.8$ | | | | | | |
| Poisson plug-in | -0.460 | 1.350 | 0.866 | 0.00 | 0.20 | 0.22 |
| Poisson cut | -0.412 | 0.153 | 0.094 | 0.25 | 0.94 | 0.94 |
| BART plug-in | -0.037 | 2.742 | 1.140 | 0.96 | 0.88 | 0.99 |
| BART cut | 0.084 | 1.946 | 0.861 | 1.00 | 1.00 | 1.00 |

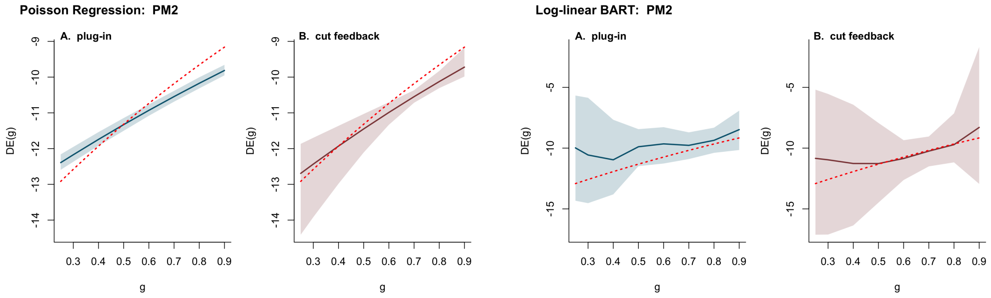


**Figure 28:** The estimated **direct effects** $(DE(g))$ for a simulation from PM2, using Poisson regression and log-linear BART regression, with a comparison between the plug-in and cutting feedback approaches.

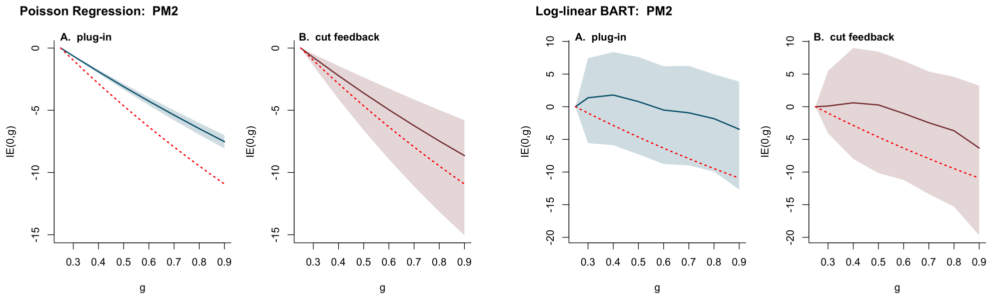


**Figure 29:** The estimated **indirect effects** $(IE(0, g))$ for a simulation from PM2, using Poisson regression and log-linear BART regression, with a comparison between the plug-in and cut feedback approaches.

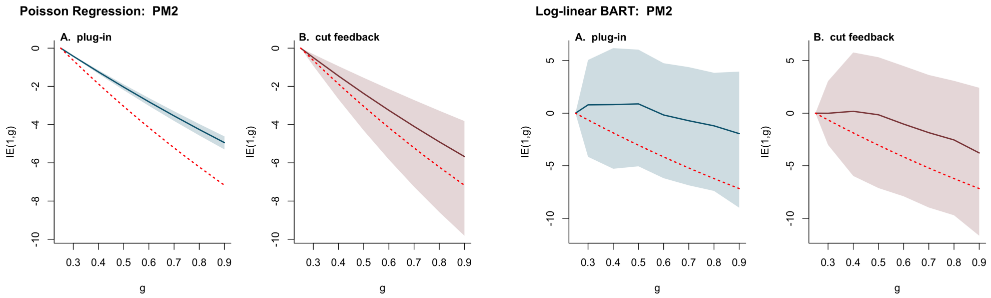


**Figure 30:** The estimated **indirect effects** $(IE(1, g))$ for a simulation from PM2, using Poisson regression and log-linear BART regression, with a comparison between the plug-in and cut feedback approaches.

#### 5.3.8 Results: PM3

Data were simulated from the following outcome model (PM3):

$$Y_i|\lambda_i \overset{ind}{\sim} \text{Poisson}(\mu_{0i}\lambda_i), \quad \text{(SM.30)}$$

$$\log\lambda_i = \begin{cases} \boldsymbol{x}_i'\boldsymbol{\beta} - 0.3z_i + 1.7\mathbb{1}_{\{g_i<0.4\}} & g_i < 0.65 \\ \exp\{-\boldsymbol{x}_i'\boldsymbol{\beta}\} - 0.25z_i - 0.1(1+z_i)\sin\{40(g_i - 0.7)\}, & 0.65 \le g_i < 0.75 \\ \boldsymbol{x}_i'\boldsymbol{\beta} - 0.5z_i - 0.5\exp\{2g_i\}, & g_i \ge 0.75 \end{cases} \quad \text{(SM.31)}$$

where $\boldsymbol{\beta} = (-4.95, -0.025, 0.325, -0.275, 0.575, 0.325, 0.225)'$ and $\mu_{0i}$ denoting the offset equal to the population size of ZCTA $i$. Here, $\log\lambda_i$ has a highly nonlinear structure, with piecewise cuts corresponding to different levels of $g_i$. Estimates of $DE(g)$ and $IE(z,g)$ were calculated for $z \in \{0,1\}$ and $g \in \{0.3, 0.4, 0.5, 0.6, 0.7, 0.8\}$, using four different estimation strategies: 1. Bayesian Poisson regression using the plug-in approach (Poisson plug-in), 2. Bayesian Poisson regression using the cut feedback approach (Poisson cut), 3. log-linear BART plug-in, and 4. log-linear BART cut. Estimated $DE(g)$ and $IE(z,g)$ curves from an example simulation are shown in Figures 31, 32, and 33.

The results from 100 simulations from PM3 are shown in Table SM.8. In general, the estimated bias in this simulation study suffers from large Monte Carlo standard error, indicating a high amount of uncertainty in each model's performance across simulations. This may be due to the nonlinearity of the causal effect curves (see the red curve in Figure 31 for an example). Consequently, general trends regarding bias are difficult to conclude. It appears that the Poisson regression cut estimates exhibit larger bias than the Poisson plug-in estimates (in all other studies, these estimates have exhibited mostly equivalent levels of bias). In contrast, with log-linear BART, the plug-in and cut feedback estimates exhibit similar levels of bias. Finally, we see that although the bias from the Poisson and log-linear BART models are variable, it appears that log-linear BART has smaller bias than the Poisson alternatives, especially as the size of $g$ grows (e.g., $g = 0.7$ and 0.8). This may indicate that as the amount of available data increases, log-linear BART is better able to identify highly nonlinear causal effect estimates. When comparing coverage, we notice that both the Poisson and log-linear BART estimates are under-covered, with Poisson coverage rates lower than the log-linear BART counterparts, and with plug-in estimates displaying the lowest coverage rates.

**Table SM.8:** Simulation study results (PM3).

| | Bias | | | Coverage | | |
|---|---|---|---|---|---|---|
| Method | DE($g$) | IE(0, $g$) | IE(1, $g$) | DE($g$) | IE(0, $g$) | IE(1, $g$) |
| $g = 0.3$ | | | | | | |
| Poisson plug-in | 15.052 | -9.474 | -9.868 | 0.01 | 0.00 | 0.00 |
| Poisson cut | 3.249 | -41.454 | -31.554 | 0.56 | 0.07 | 0.07 |
| BART plug-in | 7.066 | -0.09 | -0.143 | 0.67 | 0.76 | 0.75 |
| BART cut | 5.501 | -1.002 | -0.985 | 0.76 | 0.99 | 0.98 |
| $g = 0.4$ | | | | | | |
| Poisson plug-in | 3.274 | 20.363 | 8.192 | 0.02 | 0.03 | 0.05 |
| Poisson cut | -0.341 | -38.939 | -32.628 | 0.29 | 0.83 | 0.87 |
| BART plug-in | -4.655 | 34.659 | 22.884 | 0.67 | 0.08 | 0.16 |
| BART cut | -5.286 | 37.566 | 26.795 | 1.00 | 0.09 | 0.07 |
| $g = 0.5$ | | | | | | |
| Poisson plug-in | 2.939 | 11.760 | -0.746 | 0.02 | 0.04 | 0.03 |
| Poisson cut | 1.736 | -56.352 | -47.964 | 0.32 | 0.87 | 0.85 |
| BART plug-in | -1.575 | 26.704 | 18.009 | 0.71 | 0.27 | 0.38 |
| BART cut | -3.579 | 30.585 | 21.521 | 0.98 | 0.49 | 0.57 |
| $g = 0.6$ | | | | | | |
| Poisson plug-in | 2.717 | 6.254 | -6.475 | 0.02 | 0.01 | 0.01 |
| Poisson cut | 2.288 | -64.811 | -55.871 | 0.27 | 0.87 | 0.83 |
| BART plug-in | -2.272 | 28.202 | 18.810 | 0.35 | 0.27 | 0.38 |
| BART cut | -2.371 | 28.746 | 20.890 | 0.97 | 0.65 | 0.59 |
| $g = 0.7$ | | | | | | |
| Poisson plug-in | 6.764 | -17.975 | -26.656 | 0.00 | 0.01 | 0.01 |
| Poisson cut | 6.598 | -89.991 | -76.741 | 0.01 | 0.74 | 0.56 |
| BART plug-in | 2.449 | 15.764 | 11.092 | 0.33 | 0.52 | 0.64 |
| BART cut | 2.685 | 14.039 | 11.239 | 0.79 | 0.73 | 0.74 |
| $g = 0.8$ | | | | | | |
| Poisson plug-in | 0.227 | 9.358 | -5.861 | 0.00 | 0.01 | 0.03 |
| Poisson cut | 0.145 | -62.890 | -56.093 | 0.00 | 0.87 | 0.84 |
| BART plug-in | -0.106 | 26.678 | 19.452 | 0.81 | 0.33 | 0.39 |
| BART cut | -0.146 | 26.58 | 20.950 | 1.00 | 0.68 | 0.60 |

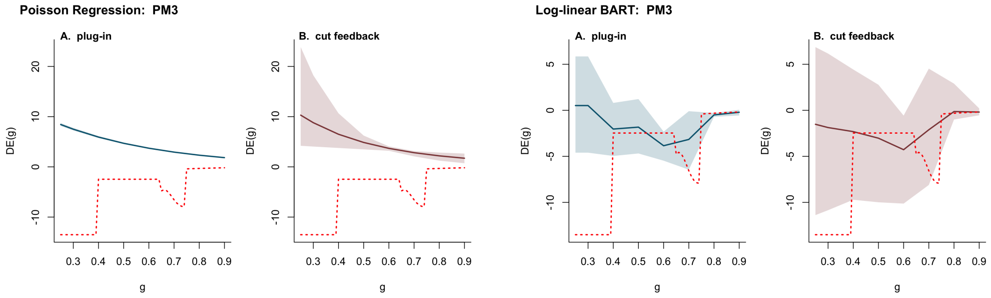


**Figure 31:** The estimated **direct effects** ($DE(g)$) for a simulation from PM3, using Poisson regression and log-linear BART regression, with a comparison between the plug-in and cutting feedback approaches.

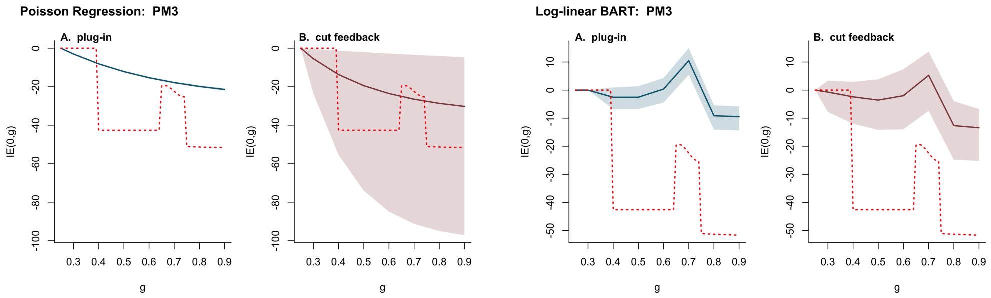


**Figure 32:** The estimated **indirect effects** ($IE(0, g)$) for a simulation from PM3, using Poisson regression and log-linear BART regression, with a comparison between the plug-in and cut feedback approaches.

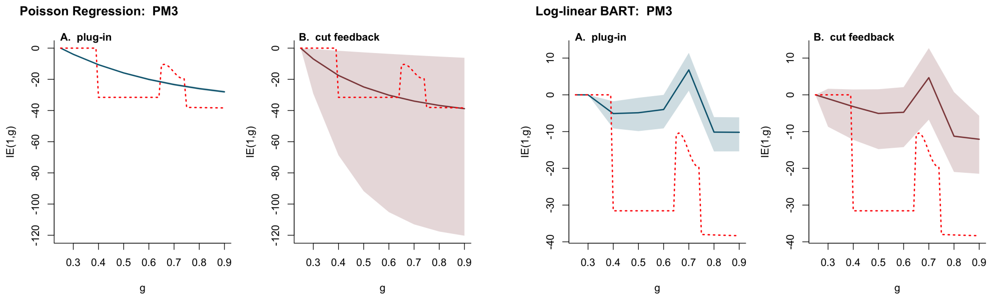


**Figure 33:** The estimated **indirect effects** ($IE(1, g)$) for a simulation from PM3, using Poisson regression and log-linear BART regression, with a comparison between the plug-in and cut feedback approaches.

# 6 Log-linear BART Tuning Parameters

Murray's [19] log-linear BART model has three main tuning mechanisms:

1. The number of trees in the BART ensemble ($m$).
2. The tree splitting prior, $p(\alpha, \beta)$.
3. The leaf prior tuning parameter, $a_0$.

We performed an analysis of the sensitivity of the causal effect estimates to the number of trees and the choice of tree splitting prior; we compare the marginal posterior standard deviation, bias, and RMSE of the estimates using different choices of $m$ and $(\alpha, \beta)$. Finally, we describe the procedure for choosing the leaf prior tuning parameter, $a_0$, when the population offset, $\mu_{0i}$, varies across outcome units; this differs from the specification in [19].

## 6.1 Number of Trees

**Conclusion:** $m = 200$ results in best RMSE performance across $DE(g)$, $IE(0, g)$, and $IE(1, g)$.

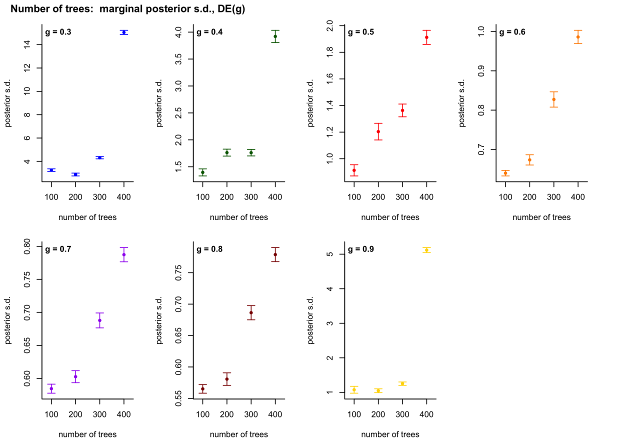


**(a)** $DE(g)$

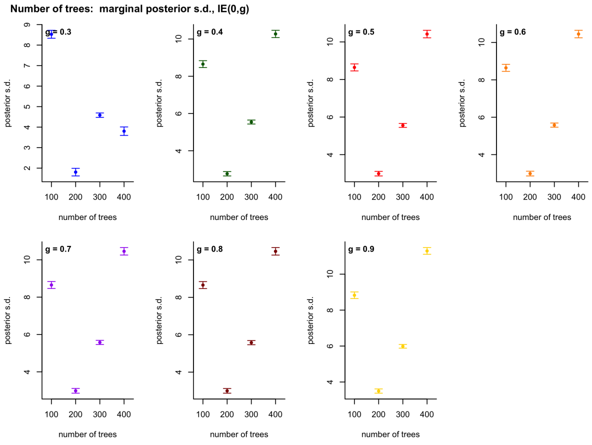


**(b)** $IE(0, g)$

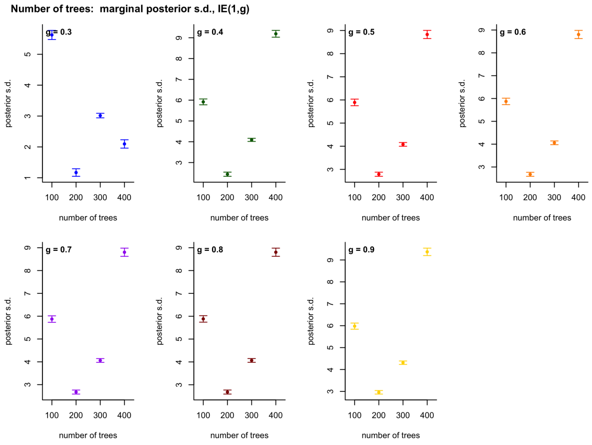


**(c)** $IE(1, g)$

**Figure 34:** A comparison of the marginal posterior standard deviation as the number of trees increases.

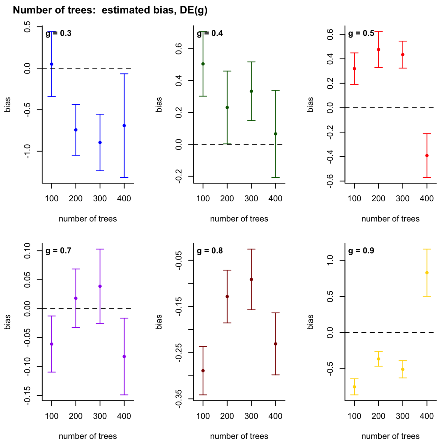


**(a)** $DE(g)$

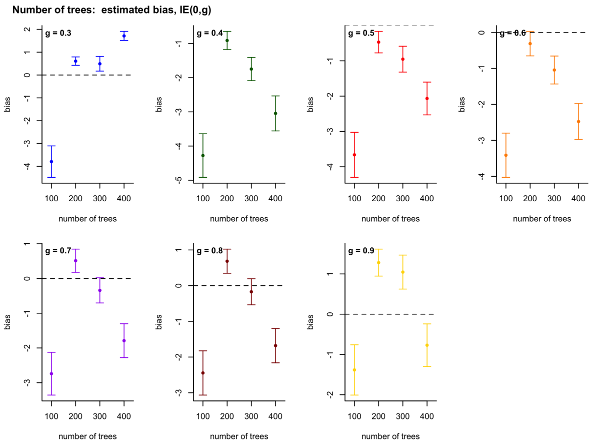


**(b)** $IE(0, g)$

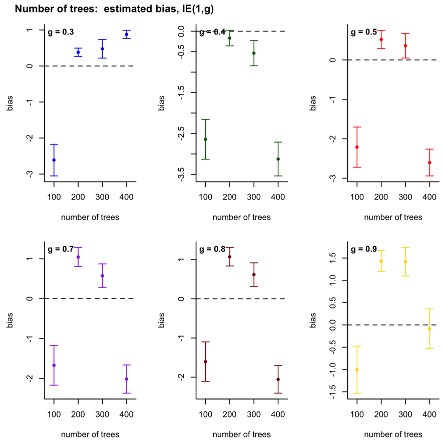


**(c)** $IE(1, g)$

**Figure 35:** A comparison of the estimated bias $(E(\hat{\theta}) - \theta)$ as the number of trees increases.

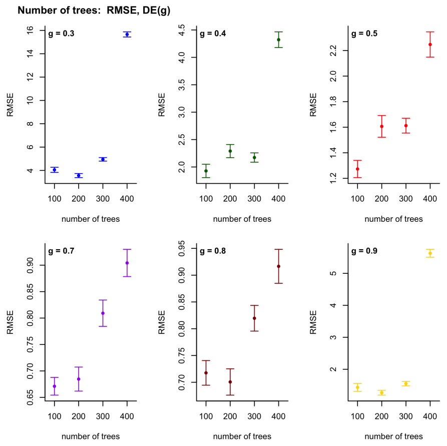


**(a)** $DE(g)$

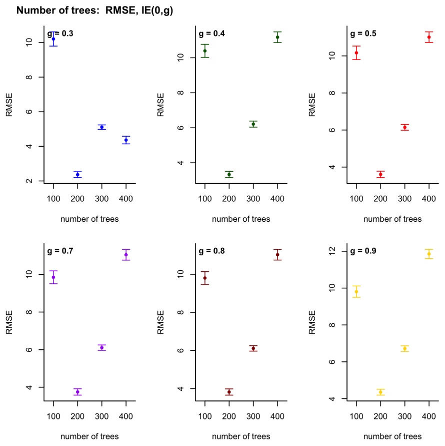


**(b)** $IE(0, g)$

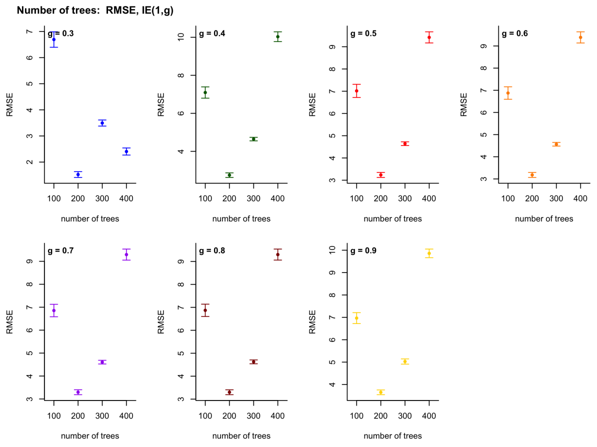


**(c)** $IE(1, g)$

**Figure 36:** A comparison of RMSE as the number of trees increases.

## 6.2 The Tree Prior: Splitting Rules

**Conclusion:** the prior distributions that favor small trees (with a depth around 2 and number of terminal nodes concentrated around 2) perform best.

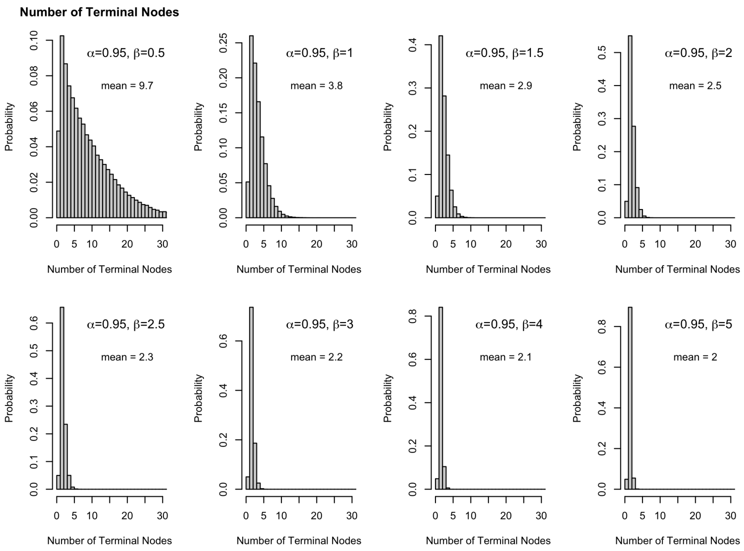


**Figure 37:** Prior distribution for the number of terminal nodes for different values of $(\alpha, \beta)$.

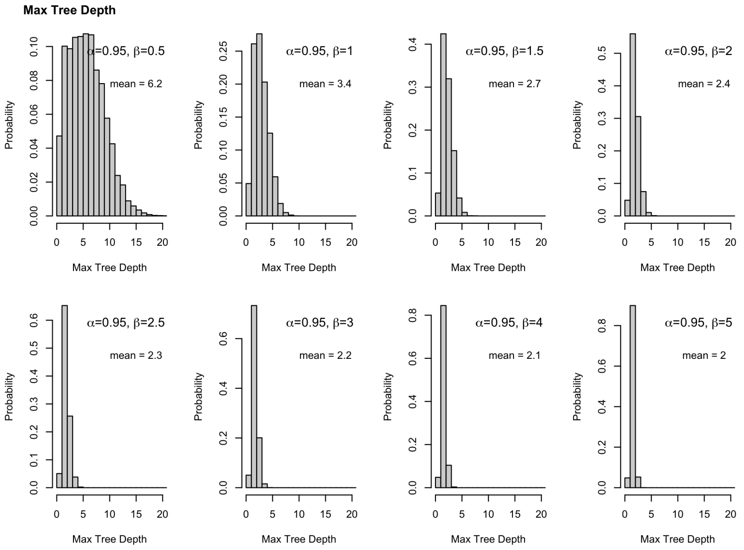


**Figure 38:** Prior distribution for maximum tree depth for different values of $(\alpha, \beta)$.

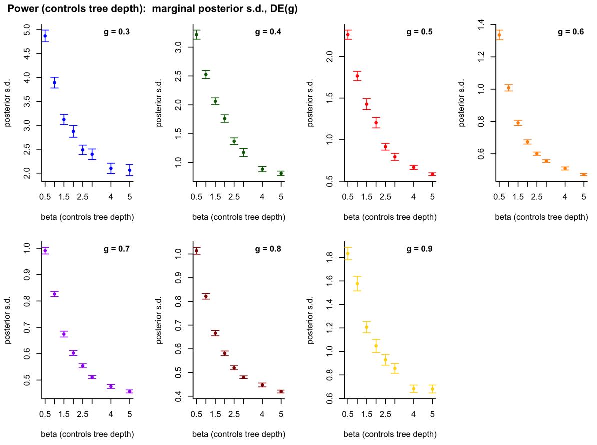


**(a)** $DE(g)$

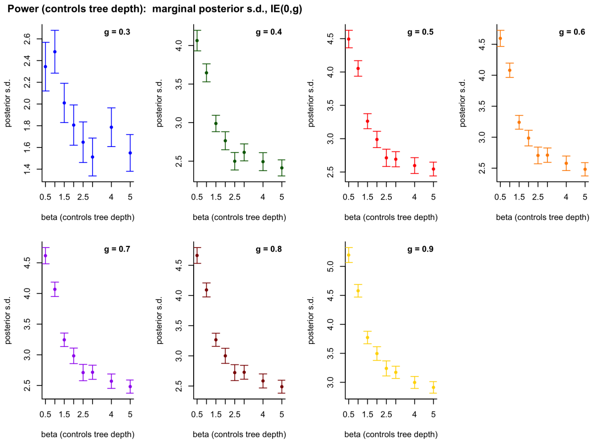


**(b)** $IE(0, g)$

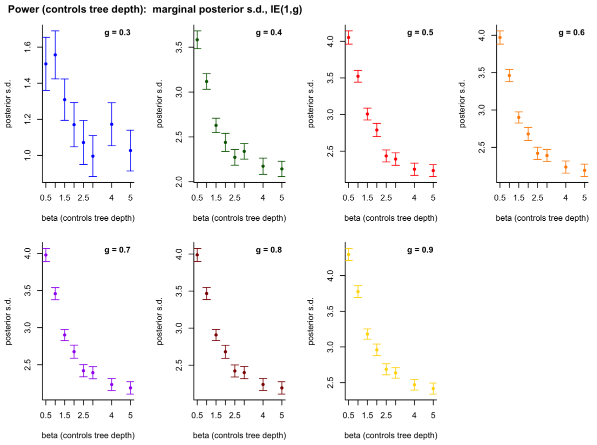


**(c)** $IE(1, g)$

**Figure 39:** A comparison of the marginal posterior standard deviation for varying levels of $\beta$; the hyperparameter determining the tree prior.

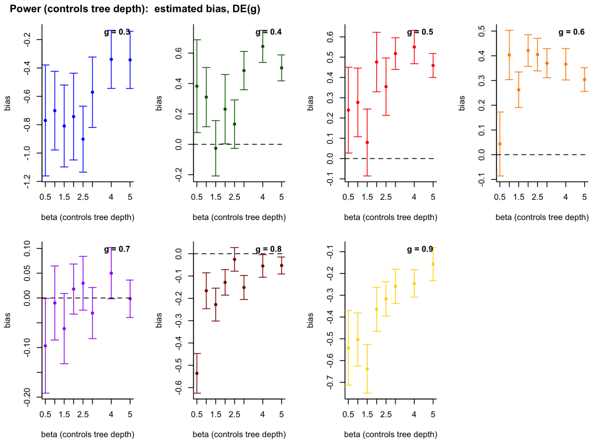


**(a)** $DE(g)$

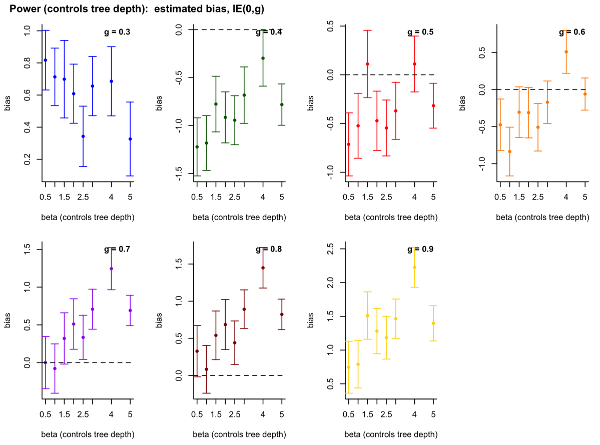


**(b)** $IE(0, g)$

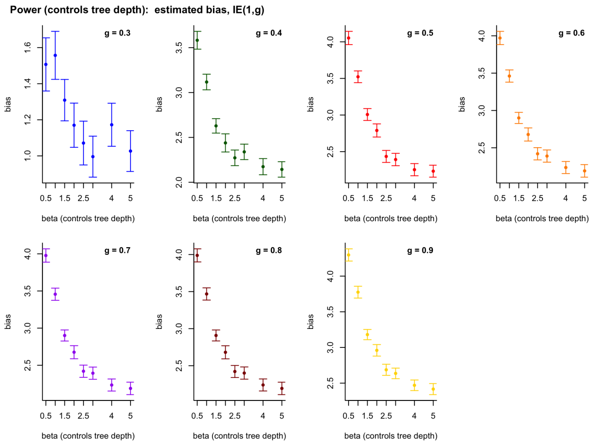


**(c)** $IE(1, g)$

**Figure 40:** A comparison of the estimated bias $(E(\hat{\theta}) - \theta)$ for varying levels of $\beta$; the hyperparameter determining the tree prior.

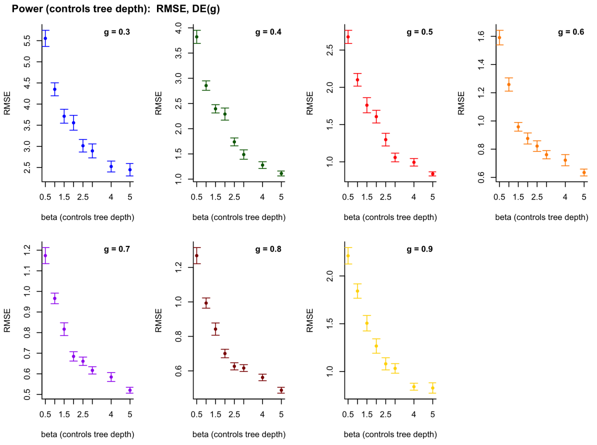


**(a)** $DE(g)$

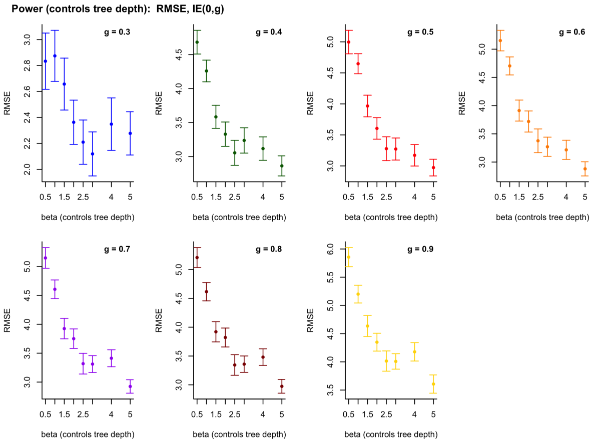


**(b)** $IE(0, g)$

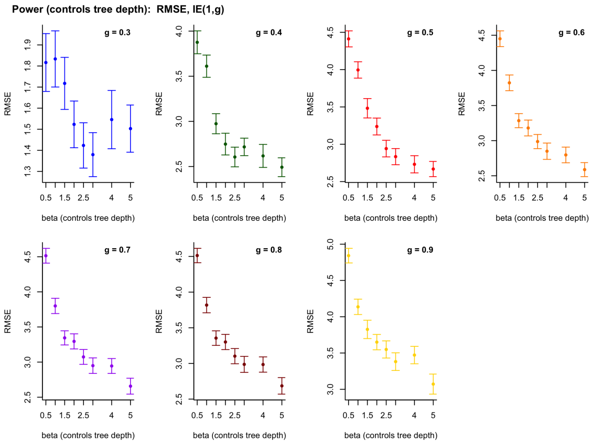


**(c)** $IE(1, g)$

**Figure 41:** A comparison of RMSE for varying levels of $\beta$; the hyperparameter determining the tree prior.

### 6.3 Leaf Prior Tuning Parameter

Murray [19] describes a default choice of $a_0$ as follows:

"*When* $\mu_{0i} = \mu_0$*, a reasonable default prior is obtained by positing a near-maximum value (or upper quantile of the empirical distribution) of* $y$*, say* $y^*$*, and setting* $a_0 = 0.5(\log(y^*) - \log(\mu_0))$*. Then* $Pr(f(\boldsymbol{x}_i) \leq y^*) \approx 0.975$ *marginally, since* $\log(f(\boldsymbol{x}_i)) \sim N(0, a_0^2)$*.*"

In our case, we have varying offset parameters (i.e., $\mu_{i0} \neq \mu_0$). We have chosen to select $a_0$ in the following way:

- $y_i^* = y_i/\mu_{0i}$, i.e., $y_i^*$ is a rate.
- $r^* =$ `quantile`$(y_i^*, p = 0.975)$; this mimics the near-maximum value specified by Murray, but for the observed *rates*.
- $\bar{r} = \frac{1}{n}\sum_{i=1}^{n} y_i^*$, the average observed rate.
- $a_0 = 0.5 * (\log(r^*) - \log(\bar{r}))$.

In other words, we define the prior with respect to the observed rates, $y_i^*$, rather than the counts, $y$. We found reasonable success when using this as the default leaf prior tuning parameter.

## 7 Estimated Upwind Effects Without Key-Associated Treatment

There may be some concern that the definition of a key-associated treatment, $Z_i$, is somewhat arbitrary, and furthermore can lead to unwanted discontinuities in the surface of $G_i$. Consequently, we have repeated our analysis without distinguishing key-associated facilities. Instead, we define a single upwind exposure, $\tilde{G}_i$, as

$$\tilde{G}_i \equiv \tilde{g}_i(\boldsymbol{S}, T) = \sum_{j \in \mathcal{J}} T_{ij} S_j / \tilde{T}_{i\cdot}^*, \tag{SM.32}$$

where $\boldsymbol{S}$ is the vector of scrubber assignments, $T$ is the source-receptor matrix defining the weighted connection between each power plant and ZCTA, and $\tilde{T}_{i\cdot}^* = \sum_{j \in \mathcal{J}} T_{ij}$. This can be viewed as a modification of the upwind exposure level considered in the original analysis, where $\tilde{G}_i$ now specifies the weighted proportion of *all* power plant facilities that have received treatment. Consequently, we define the indirect treatment, $IE(\tilde{g})$, as

$$IE(\tilde{g}) = \mu(\tilde{g}) - \mu(\tilde{g}_{min}), \tag{SM.33}$$

with $\mu(\tilde{g})$ defined in a similar way as $\mu(z, g)$ in Equation (1).

Figure 42 shows the spatial distribution of $\tilde{G}_i$ compared with the distribution of $G_i$ used in the original analysis (i.e., including key-associated treatments). In general, the two surfaces are similar, although the distribution of $\tilde{G}_i$ is smoother than that of $G_i$, due to the discontinuities introduced by $Z_i$, and the treatment levels along the Gulf Coast have flipped from near 1 when defined with $Z_i$, to around 0.5 without $Z_i$.

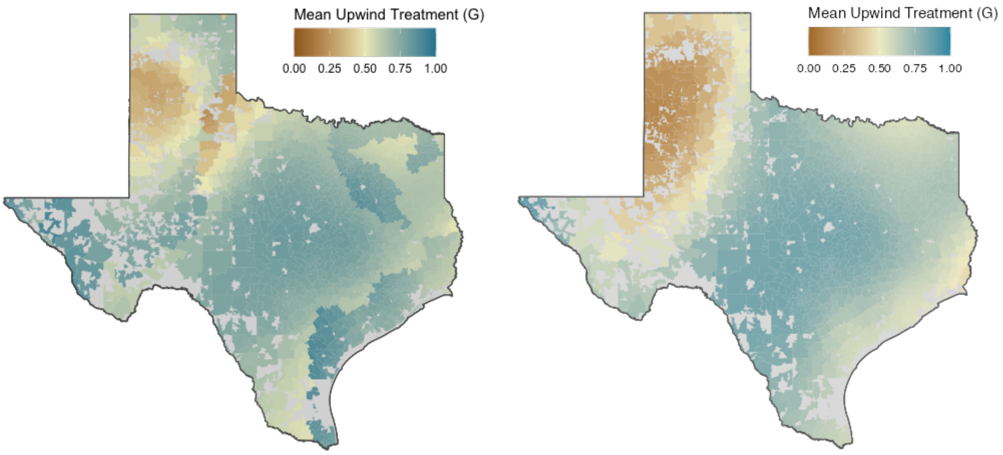


**(a)** Mean upwind treatment, $G_i$ (with $Z_i$). **(b)** Mean upwind treatment, $\tilde{G}_i$ (no $Z_i$).

**Figure 42:** A comparison of the spatial distribution of the upwind treatment levels in the analysis (a) with $Z_i$ and (b) without $Z_i$.

A comparison of the estimated upwind effects from the two analyses is shown in Figures 43 and 44. In the asthma analysis, the estimates of $IE(\tilde{g})$ and $IE(z, g)$ are very similar (Figure 43); the log-linear BART estimate without interference uncertainty propagation shows a slight reduction in the rate of ED visits as the proportion of upwind power plants increases, however, the addition of interference uncertainty pulls this estimate up towards zero. In contrast, the results from the Medicare analysis are more sensitive to the inclusion of $Z_i$ (Figure 44). In particular, the estimates

of $IE(\tilde{g})$ have narrower uncertainty bounds, and the log-linear BART estimates with and without interference uncertainty are more similar than was found in the analysis that included $Z_i$. Ultimately, we have chosen to keep the analysis with the key-associated treatment in the manuscript for the stated reasons and in part because the conclusions of the study remain relatively unchanged (i.e., in both the analysis with and without $Z_i$, after accounting for uncertainty in the interference structure, we did not find significant evidence of a reduction in all-cause mortality among Medicare benefits in Texas as the weighted proportion of scrubbers was increased).

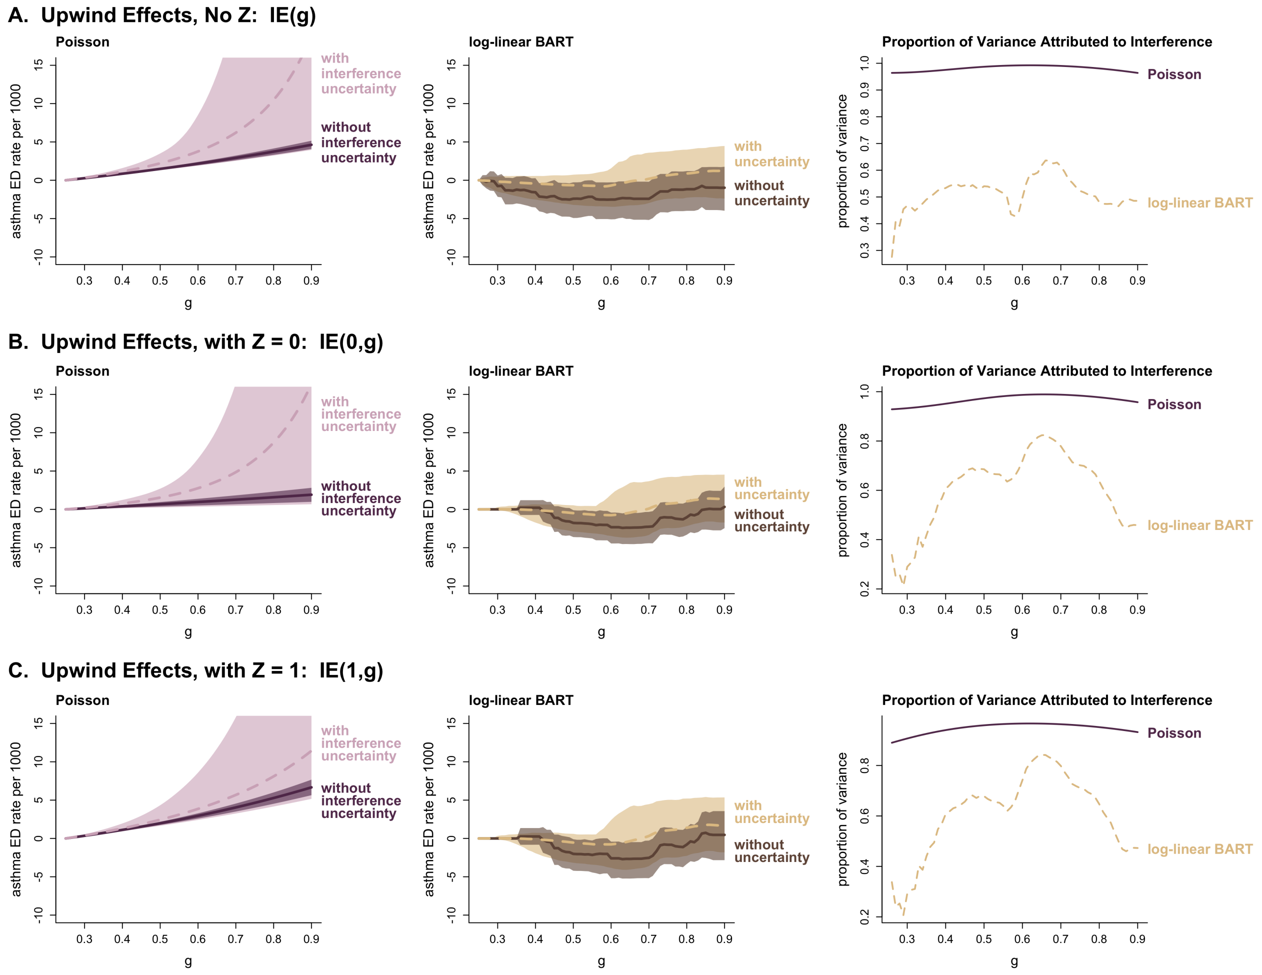


**Figure 43:** Estimated upwind effects of coal-fired power plant scrubbers on the 2016 rate of **pediatric asthma** ED visits in Texas, comparing (a) the estimated effect from an **analysis without** $Z_i$ ($IE(\tilde{g})$) to (b, c) the estimates from the analysis with $Z_i$ ($IE(0, g)$ and $IE(1, g)$).

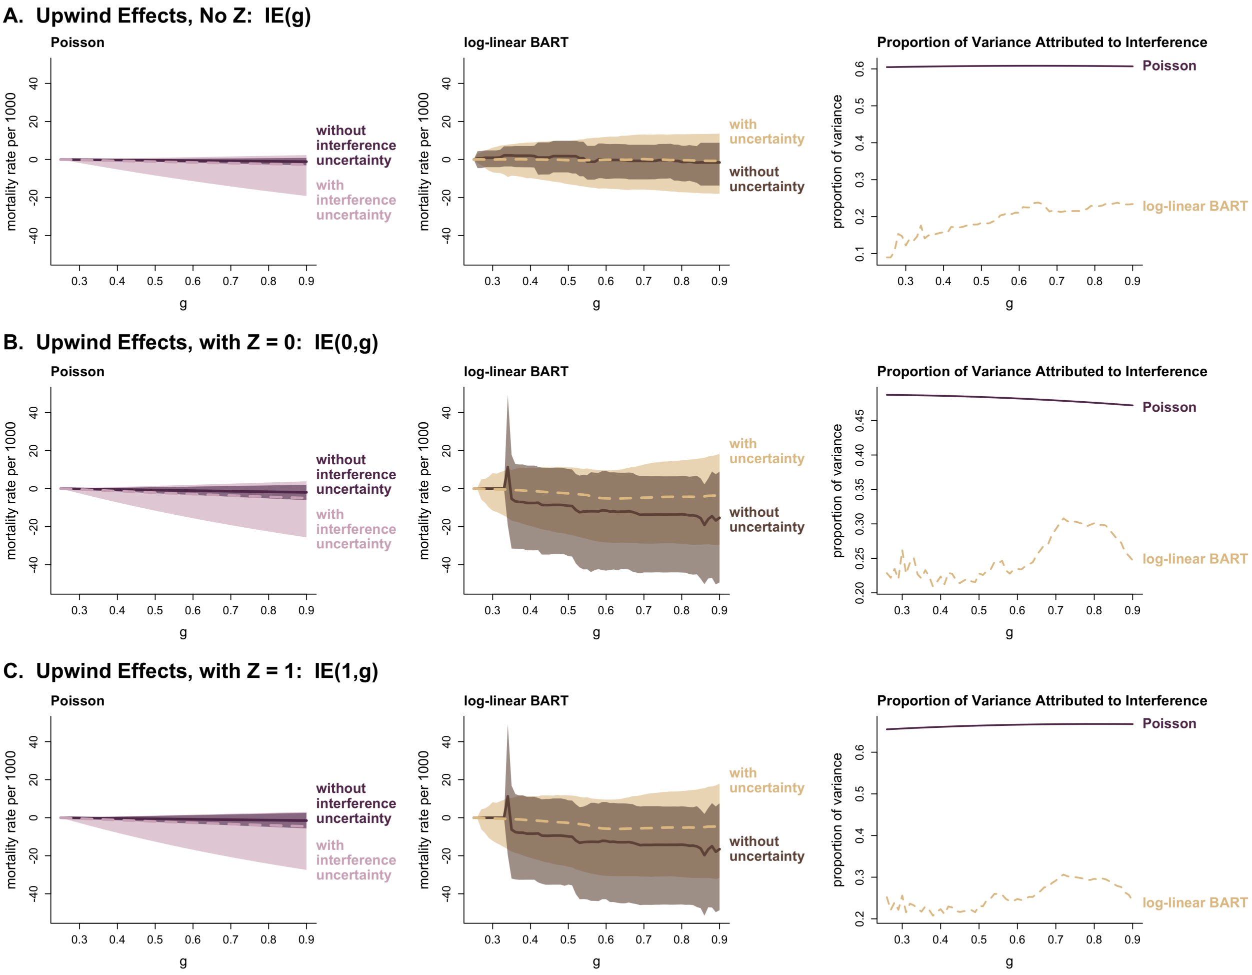


**Figure 44:** Estimated upwind effects of coal-fired power plant scrubbers on the 2016 rate of **all-cause mortality among Medicare beneficiaries** in Texas, comparing (a) the estimated effect from an **analysis without** $Z_i$ ($IE(\tilde{g})$) to (b, c) the estimates from the analysis with $Z_i$ ($IE(0,g)$ and $IE(1,g)$).

# 8 Testing for Spatial Autocorrelation

The outcomes studied in this paper are spatial (in particular, areal) observations, and it is important to consider whether spatial dependence has been appropriately accounted for in our analysis. Note that although the outcome data in Figure 1b appear to exhibit some level of spatial dependence, this may be due to the effect of spatially-varying covariates (such as population density, percent urban area, or other covariates listed in Table 1) on the rate of asthma ED visits. Consequently, we instead investigate whether the fitted models' residuals exhibit spatial autocorrelation.

Figures 45 and 46 show the (a) deviance residuals and (b) Pearson residuals from the asthma and Medicare analyses, respectively; the residuals were calculated using the posterior mean estimates from the fitted log-linear BART model. The existence of spatial autocorrelation is less obvious after adjusting for covariate and treatment effects, so we calculated Moran's $I$ and performed Moran's test for spatial autocorrelation [7]. As this test can be sensitive to the spatial-neighborhood matrix specification, we performed the test using four different spatial weights matrices: contiguous neighbors (no distance weighting), contiguous neighbors with inverse distance weighting (using ZCTA centroids), Delauney triangularization (no distance weighting), and Delauney triangularization with inverse distance weighting.

The Moran's test results for the asthma analysis are shown in Table SM.9. All p-values were estimated using the permutation test provided in the `spdep` *R* package [5]. The results indicate that there is little evidence of spatial autocorrelation in the asthma analysis; this is true when using either deviance or Pearson residuals, for each type of spatial-neighborhood matrix. Similarly, Table SM.10 show the test results for the Medicare analysis. Once again, there is not significant evidence of spatial autocorrelation in either the deviance or Pearson residuals.

Given the above results, we do not believe our analysis should be modified to account for spatial dependence. However, it is worth considering what might be done if there did exist strong evidence of spatial autocorrelation in the residuals. In principle, a spatial random effect could be added to the outcome model (i.e., the Poisson GLM could be replaced with a generalized linear mixed model (GLMM)), although doing so in the log-linear BART setting would be non-trivial. Furthermore, the source of the spatial autocorrelation must be carefully considered. If it is believed that the observed autocorrelation is indicative of an unobserved spatial confounder, we would caution against making any strong causal claims.

**Table SM.9:** The results from a permutation test for Moran's $I$ statistic (number of permutations = 999) using two types of residuals (deviance and Pearson) for the **pediatric asthma** analysis.

| | Deviance residuals | | Pearson residuals | |
|---|---|---|---|---|
| Spatial Weights Matrix | Moran's $I$ | $p$-value | Moran's $I$ | $p$-value |
| contiguous (no dist.) | 0.012 | 0.204 | -0.002 | 0.521 |
| contiguous (inv. dist.) | 0.018 | 0.139 | 0.001 | 0.447 |
| Delauney (no dist.) | 0.001 | 0.470 | -0.013 | 0.819 |
| Delauney (inv. dist.) | 0.007 | 0.315 | -0.010 | 0.753 |

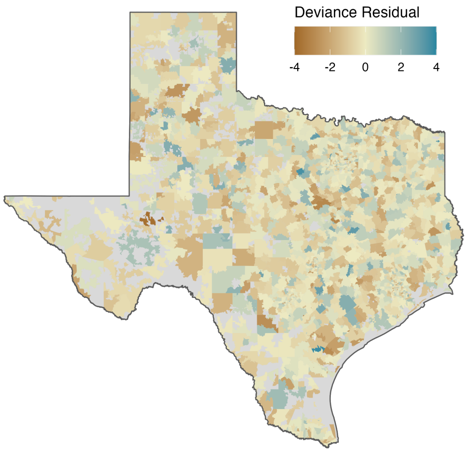


**(a)** Deviance residuals.

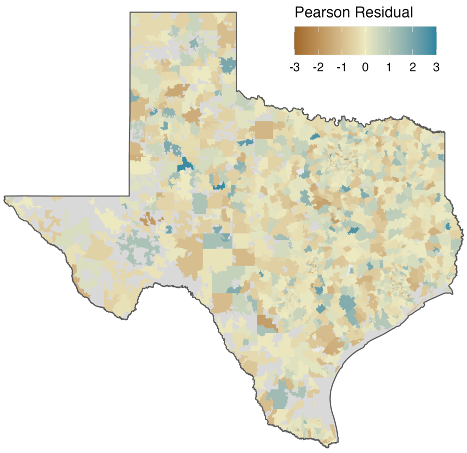


**(b)** Pearson residuals

**Figure 45:** The (a) deviance and (b) Pearson residuals from the **pediatric asthma** analysis. Residuals were calculated using the posterior mean estimates from the log-linear BART model.

**Table SM.10:** The results from a permutation test for Moran's $I$ statistic (number of permutations = 999) using two types of residuals (deviance and Pearson) for the **Medicare** analysis.

| | Deviance residuals | | Pearson residuals | |
|---|---|---|---|---|
| Spatial Weights Matrix | Moran's $I$ | $p$-value | Moran's $I$ | $p$-value |
| contiguous (no dist.) | -0.022 | 0.884 | -0.020 | 0.851 |
| contiguous (inv. dist.) | -0.021 | 0.850 | -0.020 | 0.838 |
| Delauney (no dist.) | -0.022 | 0.920 | -0.020 | 0.878 |
| Delauney (inv. dist.) | -0.021 | 0.895 | -0.020 | 0.873 |

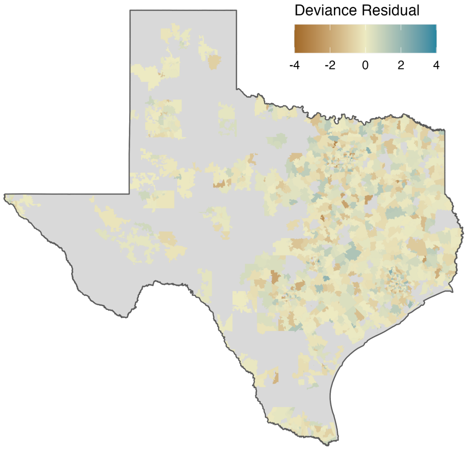


**(a)** Deviance residuals.

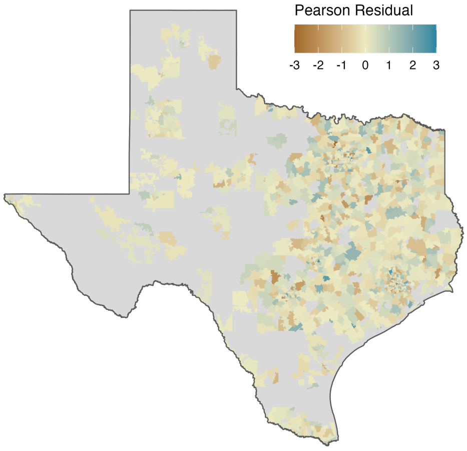


**(b)** Pearson residuals

**Figure 46:** The (a) deviance and (b) Pearson residuals from the **Medicare all-cause mortality** analysis. Residuals were calculated using the posterior mean estimates from the log-linear BART model. Note that grey areas represent ZCTAs with no eligible Medicare population.

## References


[1] Peter M. Aronow and Cyrus Samii. Estimating average causal effects under general interference, with application to a social network experiment. *The Annals of Applied Statistics*, 11(4):1912 – 1947, 2017.

[2] Peter C. Austin. Balance diagnostics for comparing the distribution of baseline covariates between treatment groups in propensity-score matched samples. *Statistics in Medicine*, 28(25):3083–3107, 2009.

[3] Peter C Austin. Assessing covariate balance when using the generalized propensity score with quantitative or continuous exposures. *Statistical Methods in Medical Research*, 28(5):1365–1377, 2019.

[4] M. J. Bayarri, J. O. Berger, and F. Liu. Modularization in Bayesian analysis, with emphasis on analysis of computer models. *Bayesian Analysis*, 4(1):119 – 150, 2009.

[5] Roger Bivand and David W. S. Wong. Comparing implementations of global and local indicators of spatial association. *TEST*, 27(3):716–748, 2018.

[6] Marta Blangiardo, Francesco Finazzi, and Michela Cameletti. Two-stage bayesian model to evaluate the effect of air pollution on chronic respiratory diseases using drug prescriptions. *Spatial and Spatio-temporal Epidemiology*, 18:1–12, 2016. Environmental Exposure and Health.

[7] Andrew D Cliff and John K Ord. *Spatial processes.* Pion Limited, 1981.

[8] Saskia Comess, Howard H Chang, and Joshua L Warren. A Bayesian framework for incorporating exposure uncertainty into health analyses with application to air pollution and stillbirth. *Biostatistics*, 08 2022.

[9] Christian Fong, Chad Hazlett, and Kosuke Imai. Covariate balancing propensity score for a continuous treatment: Application to the efficacy of political advertisements. *The Annals of Applied Statistics*, 12(1):156 – 177, 2018.

[10] Laura Forastiere, Edoardo M. Airoldi, and Fabrizia Mealli. Identification and estimation of treatment and interference effects in observational studies on networks. *Journal of the American Statistical Association*, 116(534):901–918, 2021.

[11] Alan E Gelfand and Sujit K Ghosh. Model choice: A minimum posterior predictive loss approach. *Biometrika*, 85(1):1–11, 03 1998.

[12] Tilmann Gneiting and Adrian E Raftery. Strictly proper scoring rules, prediction, and estimation. *Journal of the American Statistical Association*, 102(477):359–378, 2007.

[13] Lucas R.F. Henneman, Christine Choirat, Cesunica Ivey, Kevin Cummiskey, and Corwin M. Zigler. Characterizing population exposure to coal emissions sources in the united states using the hyads model. *Atmospheric Environment*, 203:271–280, 2019.

[14] Kosuke Imai and Marc Ratkovic. Covariate balancing propensity score. *Journal of the Royal Statistical Society: Series B (Statistical Methodology)*, 76(1):243–263, 2014.

[15] Pierre E. Jacob, Lawrence M. Murray, Chris C. Holmes, and Christian P. Robert. Better together? statistical learning in models made of modules, 2017.

[16] Duncan Lee, Sabyasachi Mukhopadhyay, Alastair Rushworth, and Sujit K. Sahu. A rigorous statistical framework for spatio-temporal pollution prediction and estimation of its long-term impact on health. *Biostatistics*, 18(2):370–385, 12 2017.

[17] David Lunn, Nicky Best, David Spiegelhalter, and Beat Neuenschwander. Combining mcmc with 'sequential' pkpd modelling. *Journal of Pharmacokinetics*, 36(1):19–38, 2009.

[18] A Marshall, D G Altman, R L Holder, and P Royston. Combining estimates of interest in prognostic modelling studies after multiple imputation: current practice and guidelines. *BMC Medical Research Methodology*, 9, 2009.

[19] Jared S. Murray. Log-linear bayesian additive regression trees for multinomial logistic and count regression models. *Journal of the American Statistical Association*, 116(534):756–769, 2021.

[20] Martyn Plummer. Cuts in bayesian graphical models. *Statistics and Computing*, 25:37–43, 2015.

[21] D B Rubin. *Multiple Imputation for Nonresponse in Surveys.* John Wiley & Sons, Ltd, 1987.

[22] David J. Spiegelhalter, Nicola G. Best, Bradley P. Carlin, and Angelika Van Der Linde. Bayesian measures of model complexity and fit. *Journal of the Royal Statistical Society: Series B (Statistical Methodology)*, 64(4):583–639, 2002.

[23] David A. Stephens, Widemberg S. Nobre, Erica E. M. Moodie, and Alexandra M. Schmidt. Causal Inference Under Mis-Specification: Adjustment Based on the Propensity Score. *Bayesian Analysis*, pages 1 – 24, 2022.

[24] G. E. Uhlenbeck and L. S. Ornstein. On the theory of the brownian motion. *Phys. Rev.*, 36:823–841, Sep 1930.

[25] J. M. Ver Hoef, E. M. Hanks, and M. B. Hooten. On the relationship between conditional (car) and simultaneous (sar) autoregressive models. *Spatial Statistics*, 25:68 – 85, 2018.

[26] Nathan B. Wikle, Ephraim M. Hanks, Lucas R. F. Henneman, and Corwin M. Zigler. A mechanistic model of annual sulfate concentrations in the united states. *Journal of the American Statistical Association*, 0(0):1–12, 2022.

[27] Corwin Zigler, Laura Forastiere, and Fabrizia Mealli. Bipartite interference and air pollution transport: Estimating health effects of power plant interventions, 2020.

[28] Corwin M. Zigler, Krista Watts, Robert W. Yeh, Yun Wang, Brent A. Coull, and Francesca Dominici. Model feedback in bayesian propensity score estimation. *Biometrics*, 69(1):263–273, 2013.

[29] Corwin Matthew Zigler. The central role of bayes' theorem for joint estimation of causal effects and propensity scores. *The American Statistician*, 70(1):47–54, 2016.
